# Supplementary material for: Variational Transformer Networks for Layout Generation
Source: arXiv:2104.02416 source file (2021-04-06)
Supplement: Supplementary file 1 [file model_details_and_optimization.tex]

\paragraph{Encoder} The encoder is similar for both model variants, and its input is the entire sequence of elements. First, the elements are transformed by a feed-forward layer with output dimensionality $d_{model}$. Afterwards, we use a series of the multi-head self-attention layers proposed by \cite{DBLP:conf/nips/VaswaniSPUJGKP17} to model many-to-many relationships between elements. These consist of three independent linear layers whose outputs are the $Q$, $K$ and $V$ values of the scaled dot-product attention operation:
\begin{align}
    \text{Attention(Q,K,V}) = \text{softmax}\left(\frac{Q^TK}{d_k}\right)\cdot V
\end{align}
Multiple instances (``heads'') of this operation perform in parallel, with a linear layer aggregating the final output. A point-wise feed-forward network refines the output for each element in the sequence.
Since our data domain is significantly less diverse than a language modeling task, we use a smaller configuration. In particular, we use 4 self-attention blocks instead of 6 on both decoder and encoder, with $d_\text{model}=512$. In practice, we find that reducing the original number of heads $n_{heads}=8$ or the hidden size of the point-wise feed-forward layers $d_{ff}=2048$ harms the quality of the generations.

\paragraph{Decoder} As in the encoder, we use a set of self-attention blocks as decoder. We also use 4 self-attention blocks with $d_\text{model}=512$. The values for $n_{heads}=8$ and $d_{ff}=2048$ are identical to the original Transformer. In the autoregressive case, the vector $\mathbf{z}$ is the single piece of information that the decoder receives from the encoder, as such, we make some changes to the original decoder. We define two distinct inputs: $\mathbf{z}$, a representation of the entire document, and $\mathbf{x}_t$, the partial set of already generated elements at step $t$. $\mathbf{x}_t$ grows in size during the autoregressive decoding, as new elements are appended to it, starting as a single \BOS{} token, common to all layouts. Contrary to the original decoder formulation, the encoder information is not used as query and key values for the self-attention layers, but rather is simply prepended to $\mathbf{x}_t$. In the \textbf{non-autoregressive} case \janis{Complete}

Similarly to the original Transformer, we use dropout \cite{JMLR:v15:srivastava14a} and layer normalization \cite{ba2016layer} after the multi-head attention and point-wise segments in both encoder and decoder. Note that since our data already encodes positional information, there is no need for the positional encodings used in the original Transformer.

\paragraph{Data format} Each of our datasets $\mathbf{X}$ consists of documents with different elements $t$ (such as text boxes, figures, types of furniture or \ac{ui} elements), which have a category $c \in C$ as well as a bounding box annotation (parameterized as $\left(x_\text{center}, y_\text{center}, \text{width}, \text{height}\right)$). In general, bounding boxes are always assumed to be axis-aligned rectangles. We use different formats for input and output. For the output, given a series of document elements with their category, location and size, we divide the normalized coordinate space into a grid of size $H \times W$, and associate each vertical and horizontal coordinate value to a discretized entry in $1\dots H$ and $1\dots W$ respectively. Each property of an element can be thus parameterized as a one-hot vector. Contrary to \cite{2020arXiv200614615G}, we use a single vector to represent an element instead of 5, simply by concatenating each component. We use two additional classes \BOS{} and \EOS{} to determine the beginning and end of a sequence (necessary for the autoregressive step), and encode the category as a one-hot vector. Thus, each element in a document is represented by a vector of size $(C+2)+2\times(H+W)$. This representation reduces the memory footprint and the number of autoregressive steps, and in practice we observe an improvement in the quality and diversity of the network outputs.
Each document is thus a sequence of $n+2$ elements, where the \BOS{} and \EOS{} auxiliary vectors have zeros everywhere except in the class segment.
We arrange the elements in a document in top-left to bottom-right order.
The input to our model follows the same convention, but in a continuous format. \ie, each element is encoded as a one-hot class vector plus four real coordinates $\in [0, 1]$ (thus the total length is $(C+2) + 4$.
We briefly explore the possibility of using the continuous format as output. As we show in the supplementary, this performs significantly worse than the discrete case, and settle for this format in our final experiments.

\paragraph{Reparameterization trick} The output of the encoder is passed through an additional pair of feed-forward layers that compute the mean $\mu$ and the variance $\sigma^2$ of a normal distribution used to sample from the decoder. Since a gradient cannot flow through a random node, the following \textit{reparameterization trick} is used to enable backpropagation w.r.t. $\phi,\theta$:
\begin{align}
    z = \mu + \sigma \cdot \epsilon, \epsilon \sim \mathcal{N}(0, 1)
\end{align}

\paragraph{Optimization} We use the categorical cross-entropy loss as the reconstruction term in \autoref{eq:betaelbo} between each segment of an element vector.
We use Adam \cite{DBLP:journals/corr/KingmaB14} as our optimizer. The choice for $\beta$ in \autoref{eq:betaelbo} is often difficult. Similarly to \cite{DBLP:conf/conll/BowmanVVDJB16,DBLP:conf/ijcnn/LiuL19a}, we start at $\beta=0$, and slowly increase its value by \begin{align}
    \beta = \frac{1}{1+e^{-k\cdot i + b}}
\end{align}
Where $k=0.0025$, $b=6.25$ and $i$ is the current number of iterations.

\paragraph{Sampling} Our goal is to sample new layouts from the decoder by feeding a $\mathbf{z}$ vector that encodes a representation of a document. We assume that values for $\mathbf{z}$ can be sampled from a continuous prior distribution $p_\theta(\mathbf{z})$, in our case $\mathcal{N}(0,1)$. Our goal is to use the conditional decoder $p_{\theta}(x|z)$ for sampling.

\subsection{Implementation Details}

We implement our method using Tensorflow 2 \cite{tensorflow2015-whitepaper} using an NVIDIA V100 GPU for acceleration. We train using the Adam optimizer with a batch size of \todo{Settle on batch sizes}
\todo{Complete}
