# Supplementary material for: Variational Transformer Networks for Layout Generation
Source: arXiv:2104.02416 source file (2021-04-06)
Supplement: Supplementary file 2 [file sota_comparison.tex]

\clearpage
\onecolumn

\section{Comparison with existing methods}
In this section we compare qualitative results on existing methods such as [16] and [9] with ours on multiple datasets.

\subsection{PubLayNet}
\begin{figure}[h]
    \setlength{\tabcolsep}{2pt}
    \newlength{\qualitativeComparisonWidthPubLayNet}
    \setlength{\qualitativeComparisonWidthPubLayNet}{0.168\linewidth}
    \centering
    \begin{tabular}{c|c}
        \rotatebox{90}{\hspace{0.8cm} [16]} &  \\
        \rotatebox{90}{\hspace{0.8cm} [9]} &  \\
        \rotatebox{90}{\hspace{0.8cm} Ours}
    \end{tabular}    
    
    \caption{Comparison on PubLayNet}
    \label{fig:sota_comparison_publaynet}
\end{figure}

\subsection{RICO}
\subsection{COCO}

\begin{figure}[b]
    \setlength{\tabcolsep}{2pt}
    \newlength{\qualitativeComparisonWidth}
    \setlength{\qualitativeComparisonWidth}{0.168\linewidth}
    \newlength{\qualitativeComparisonWidthCoco}
    \setlength{\qualitativeComparisonWidthCoco}{0.228\linewidth}
    \centering
    \begin{tabular}{ccc|cc}
\rotatebox{90}{\hspace{0.8cm} [16]} &
\includegraphics[width=\qualitativeComparisonWidthCoco]{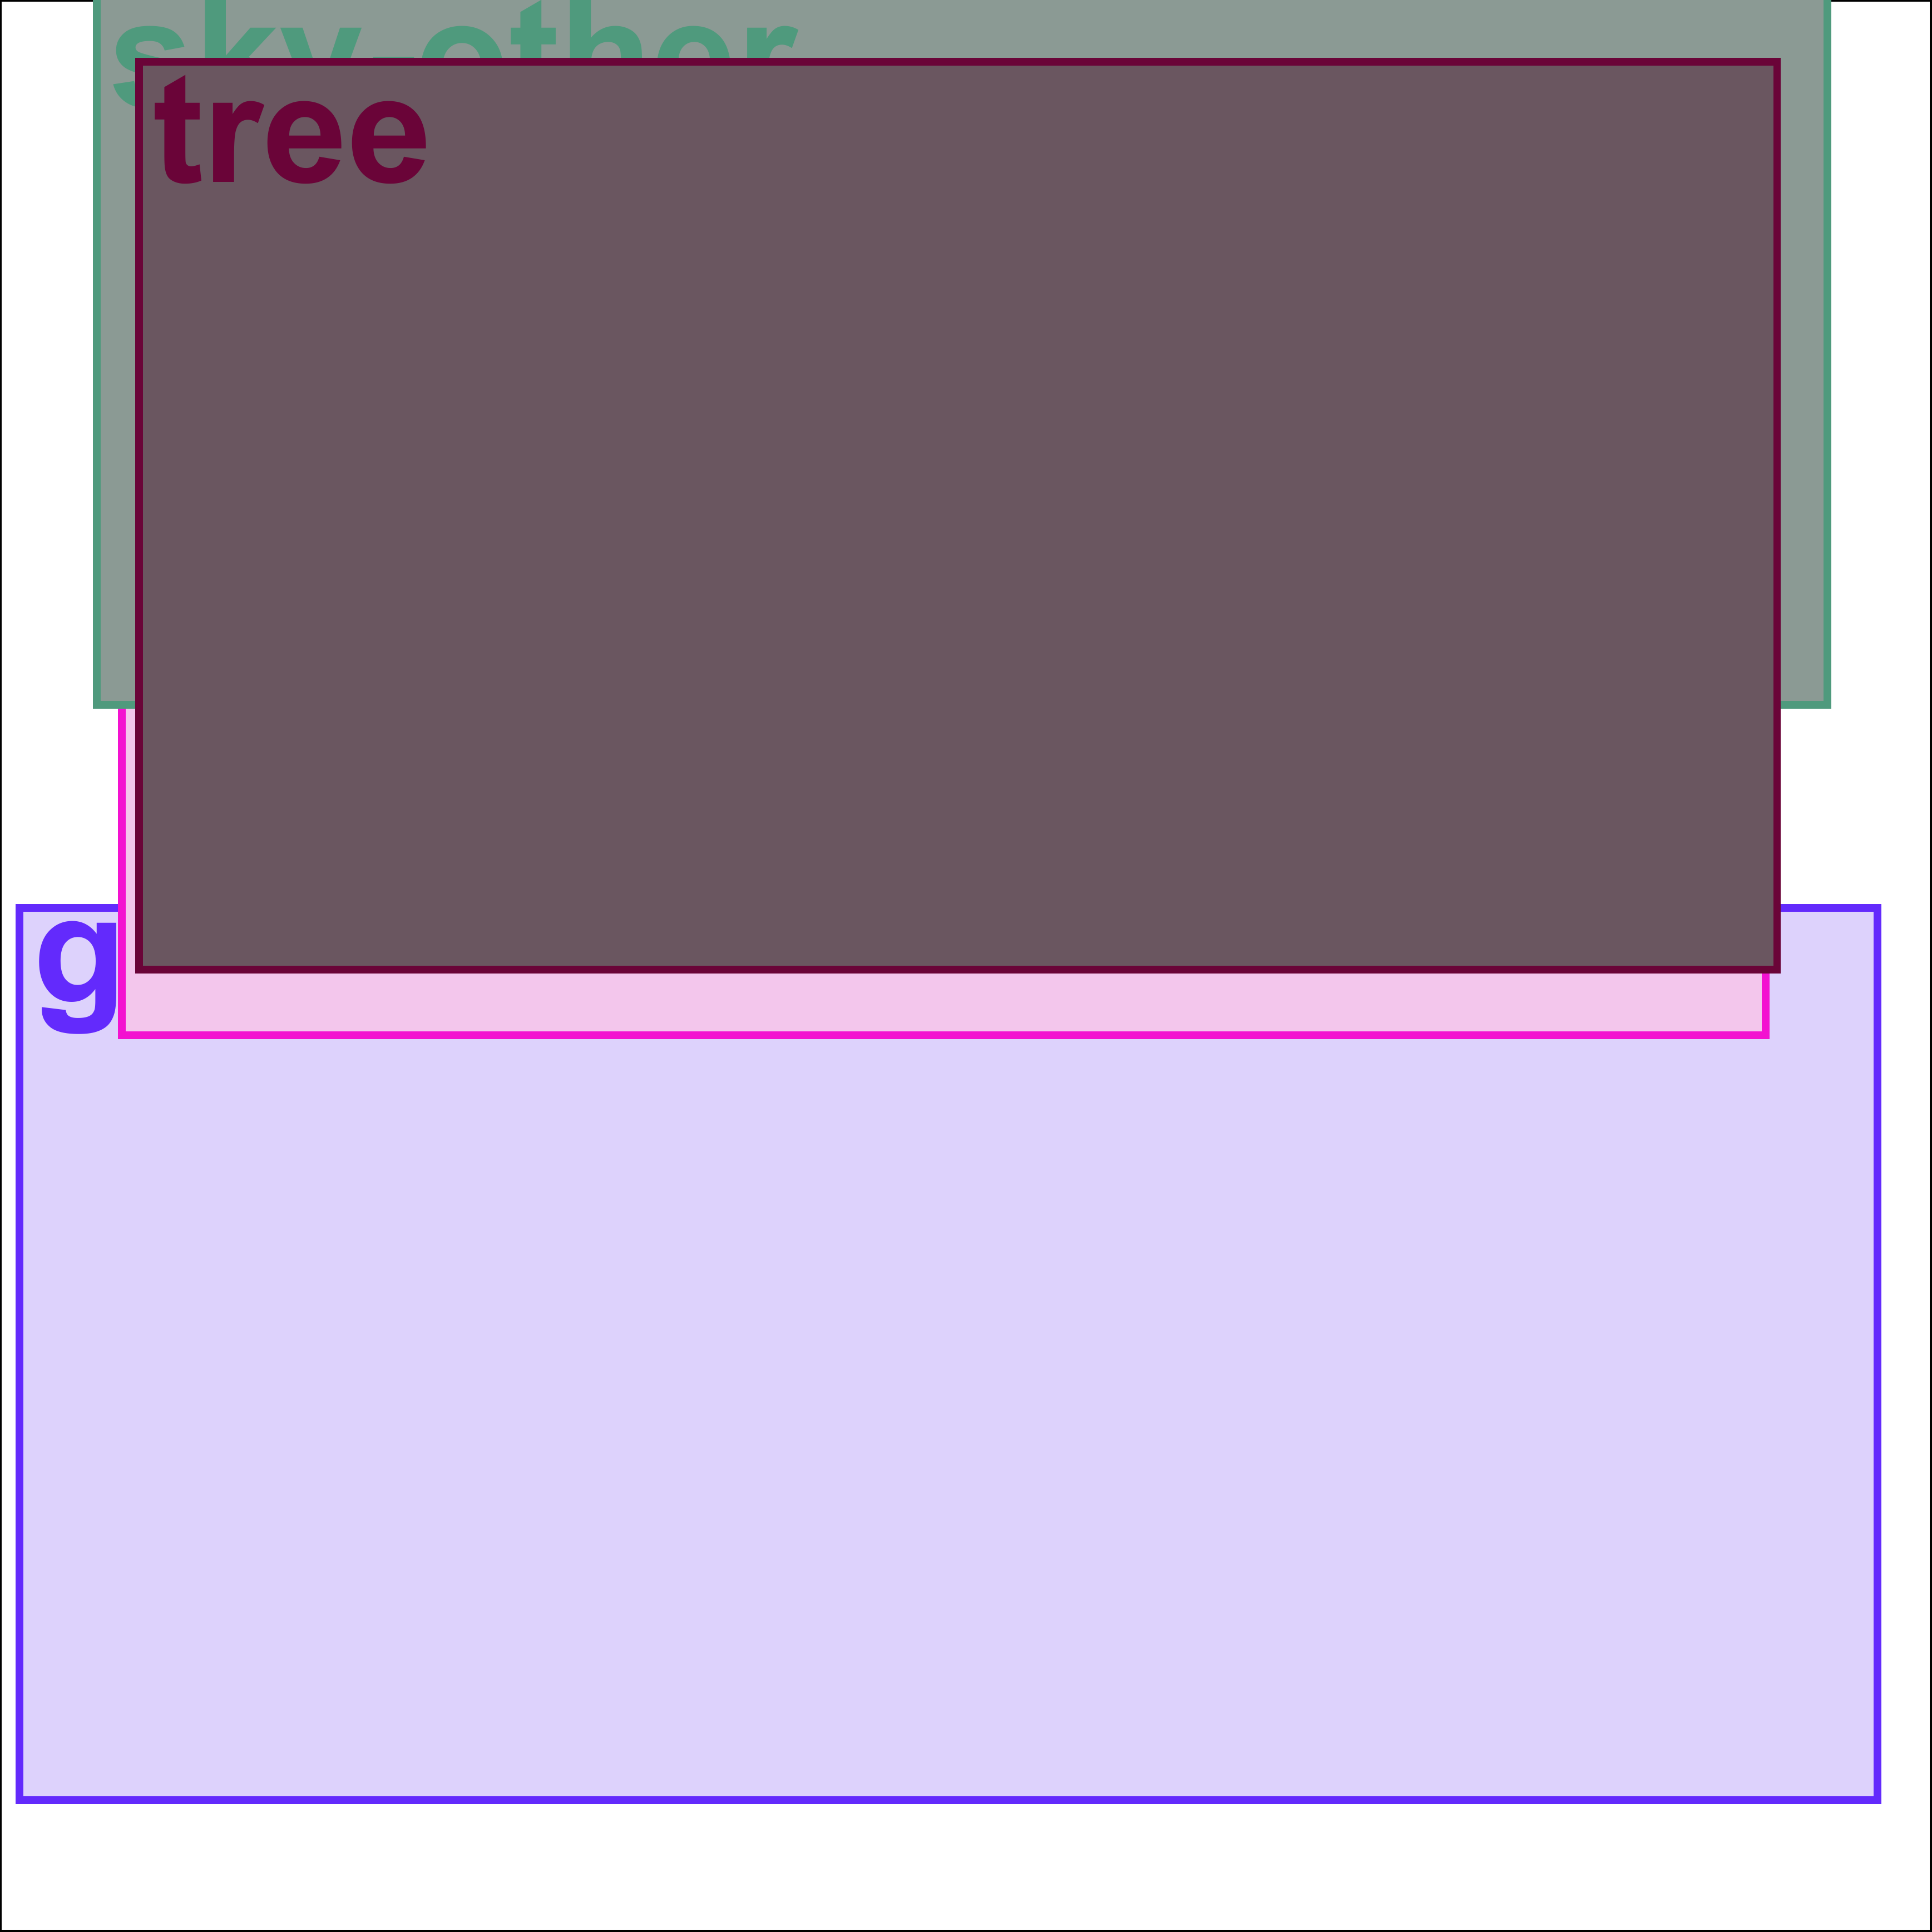} &
\includegraphics[width=\qualitativeComparisonWidthCoco]{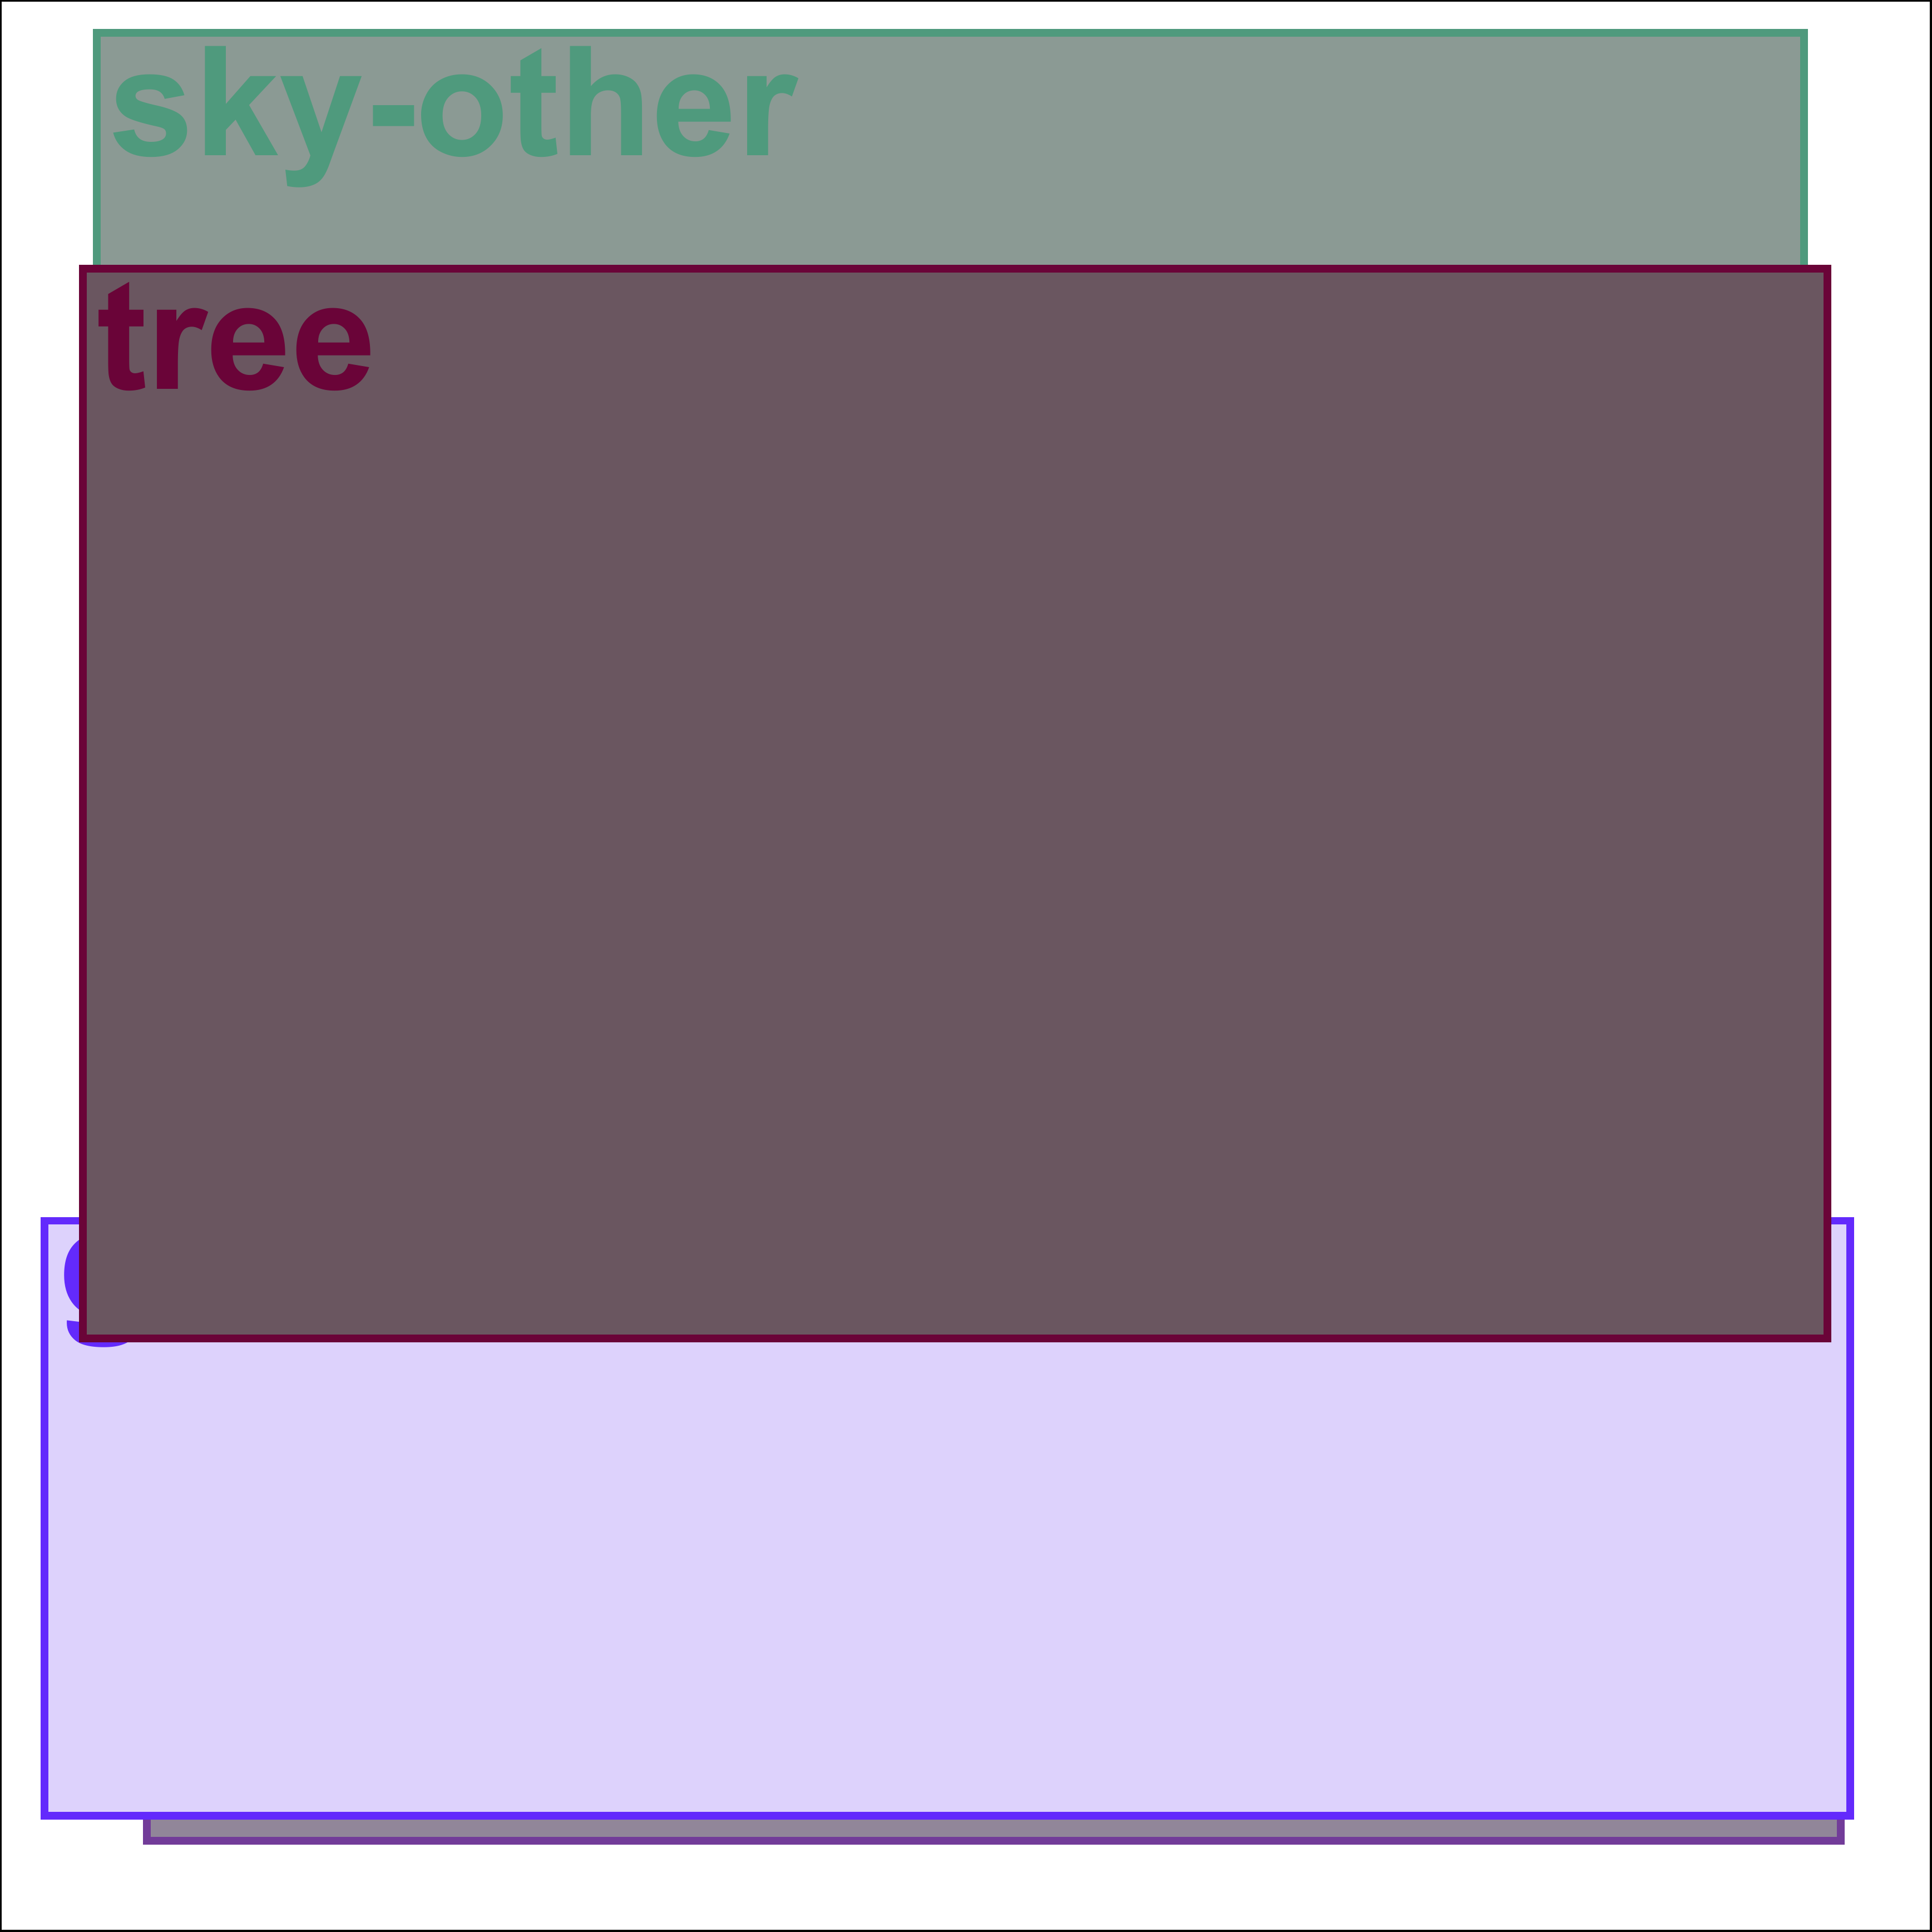} &
\includegraphics[width=\qualitativeComparisonWidth]{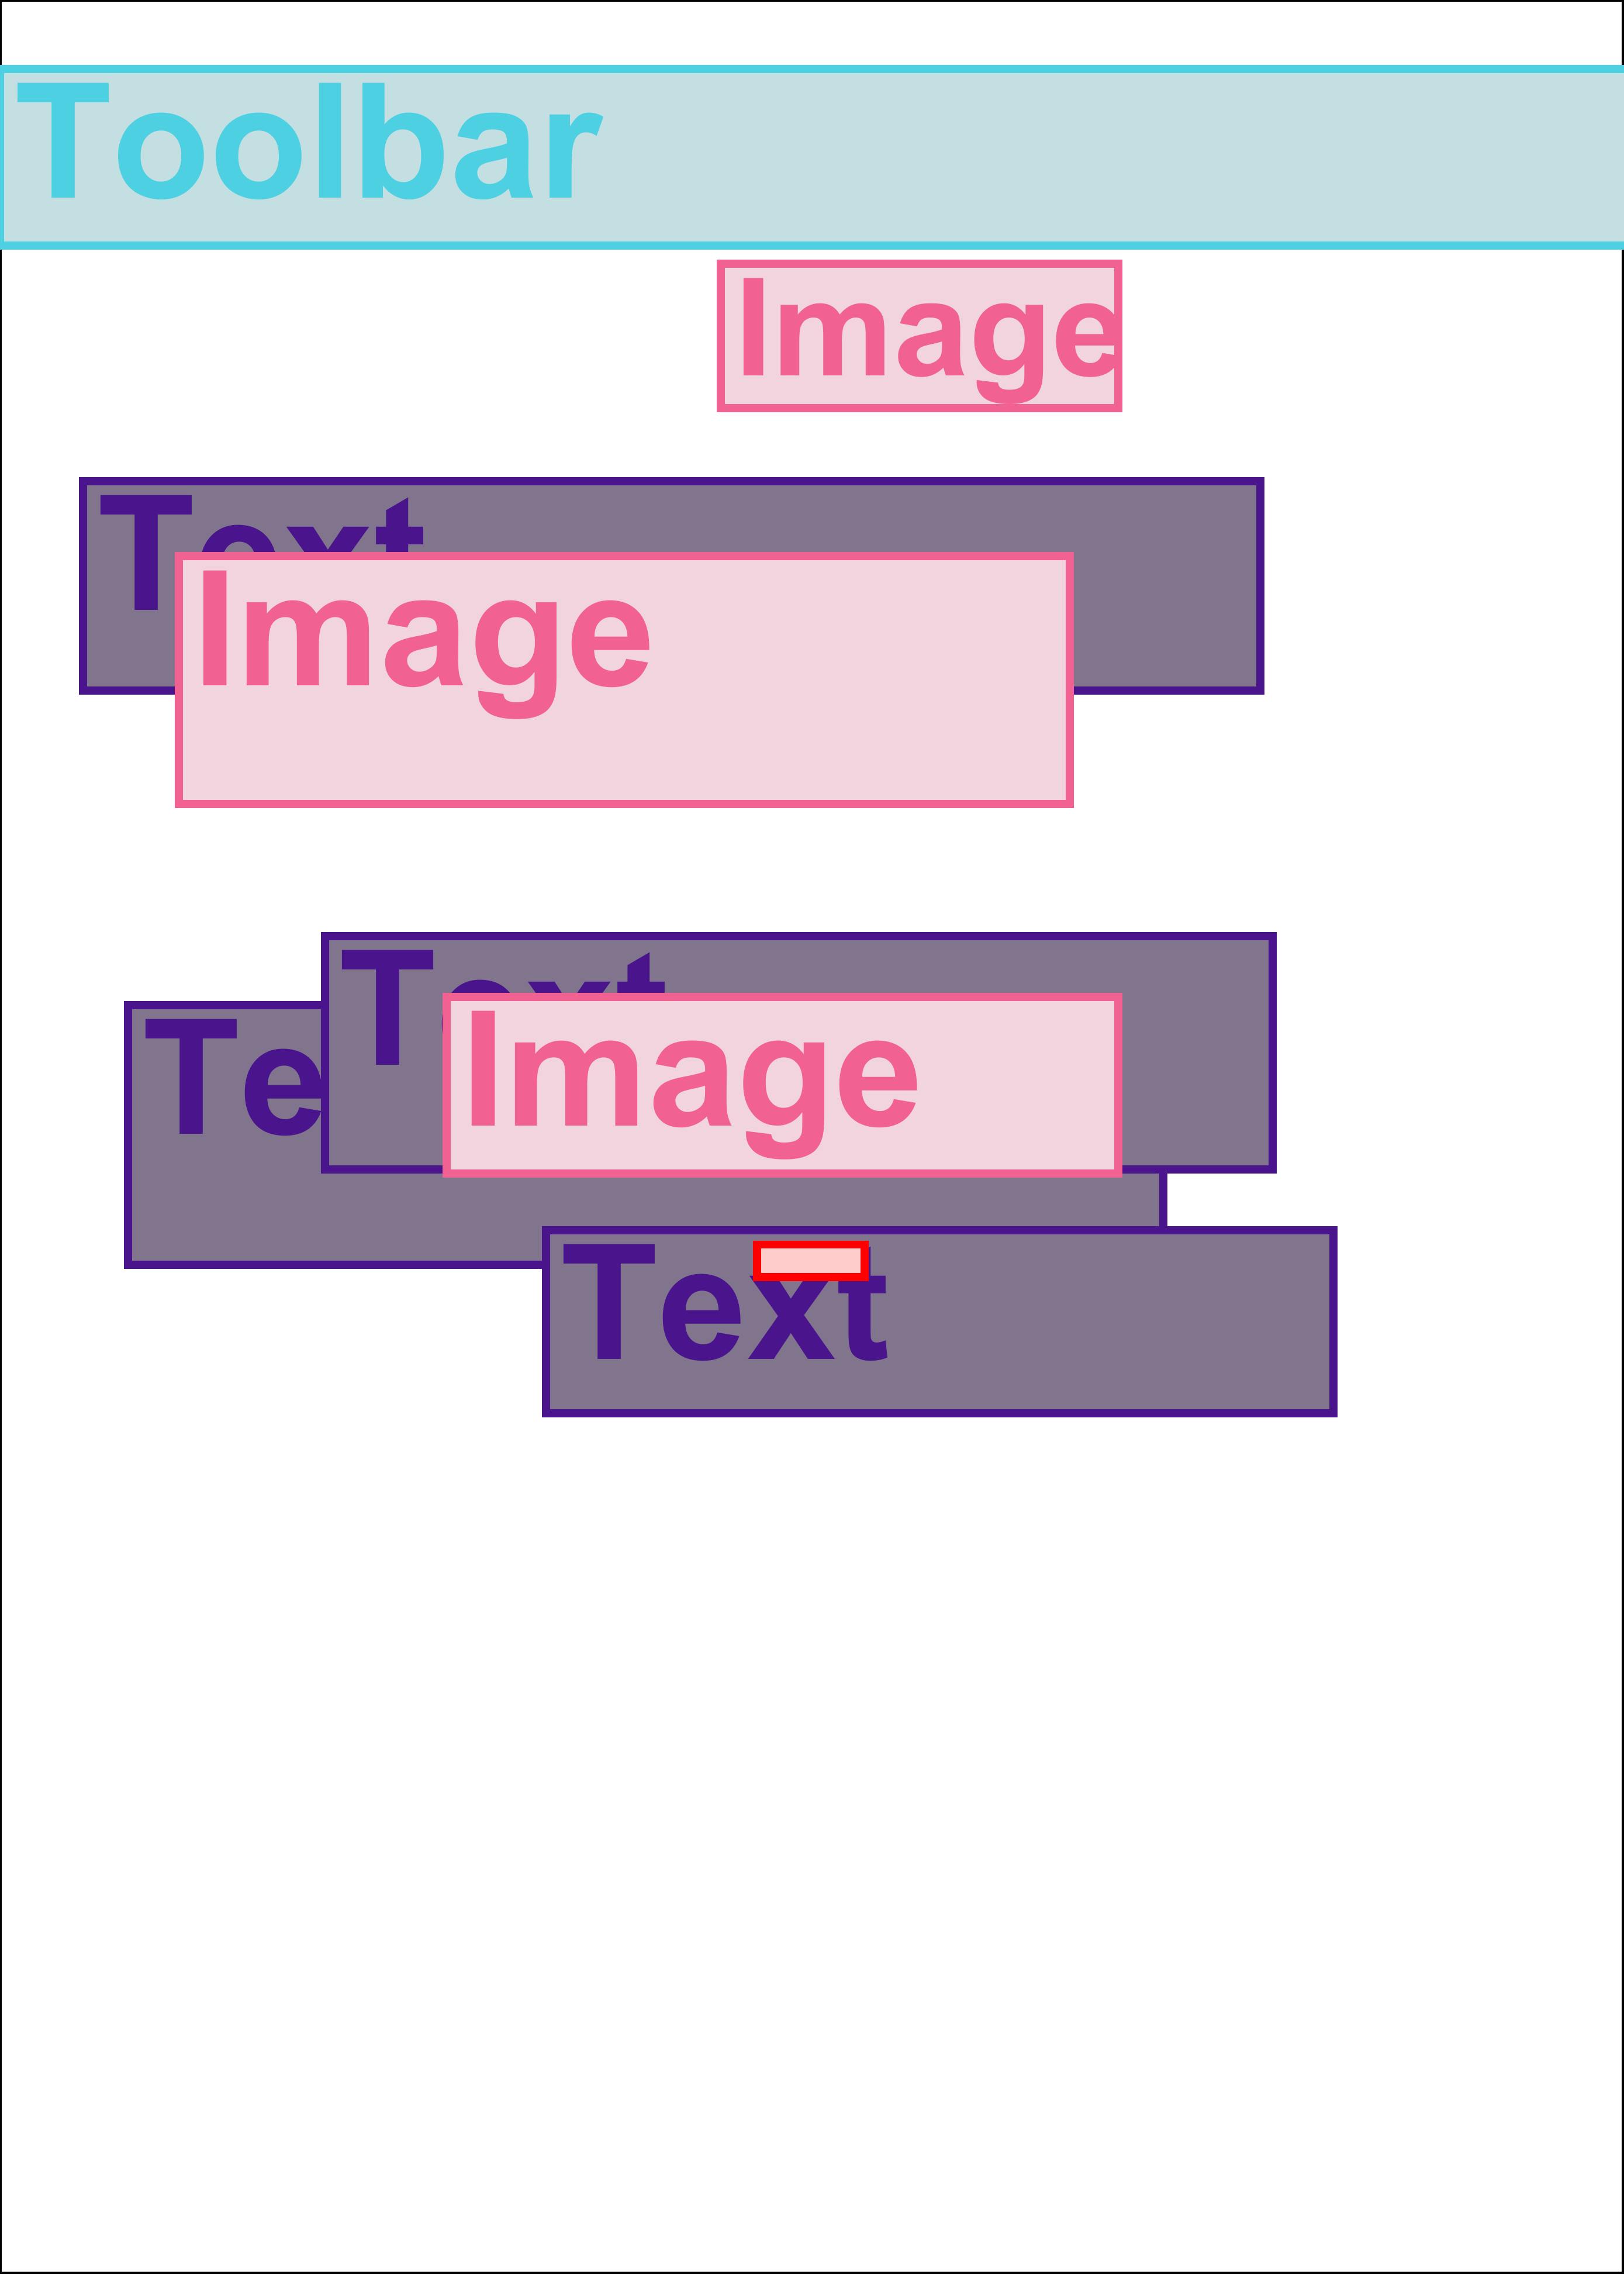} &
\includegraphics[width=\qualitativeComparisonWidth]{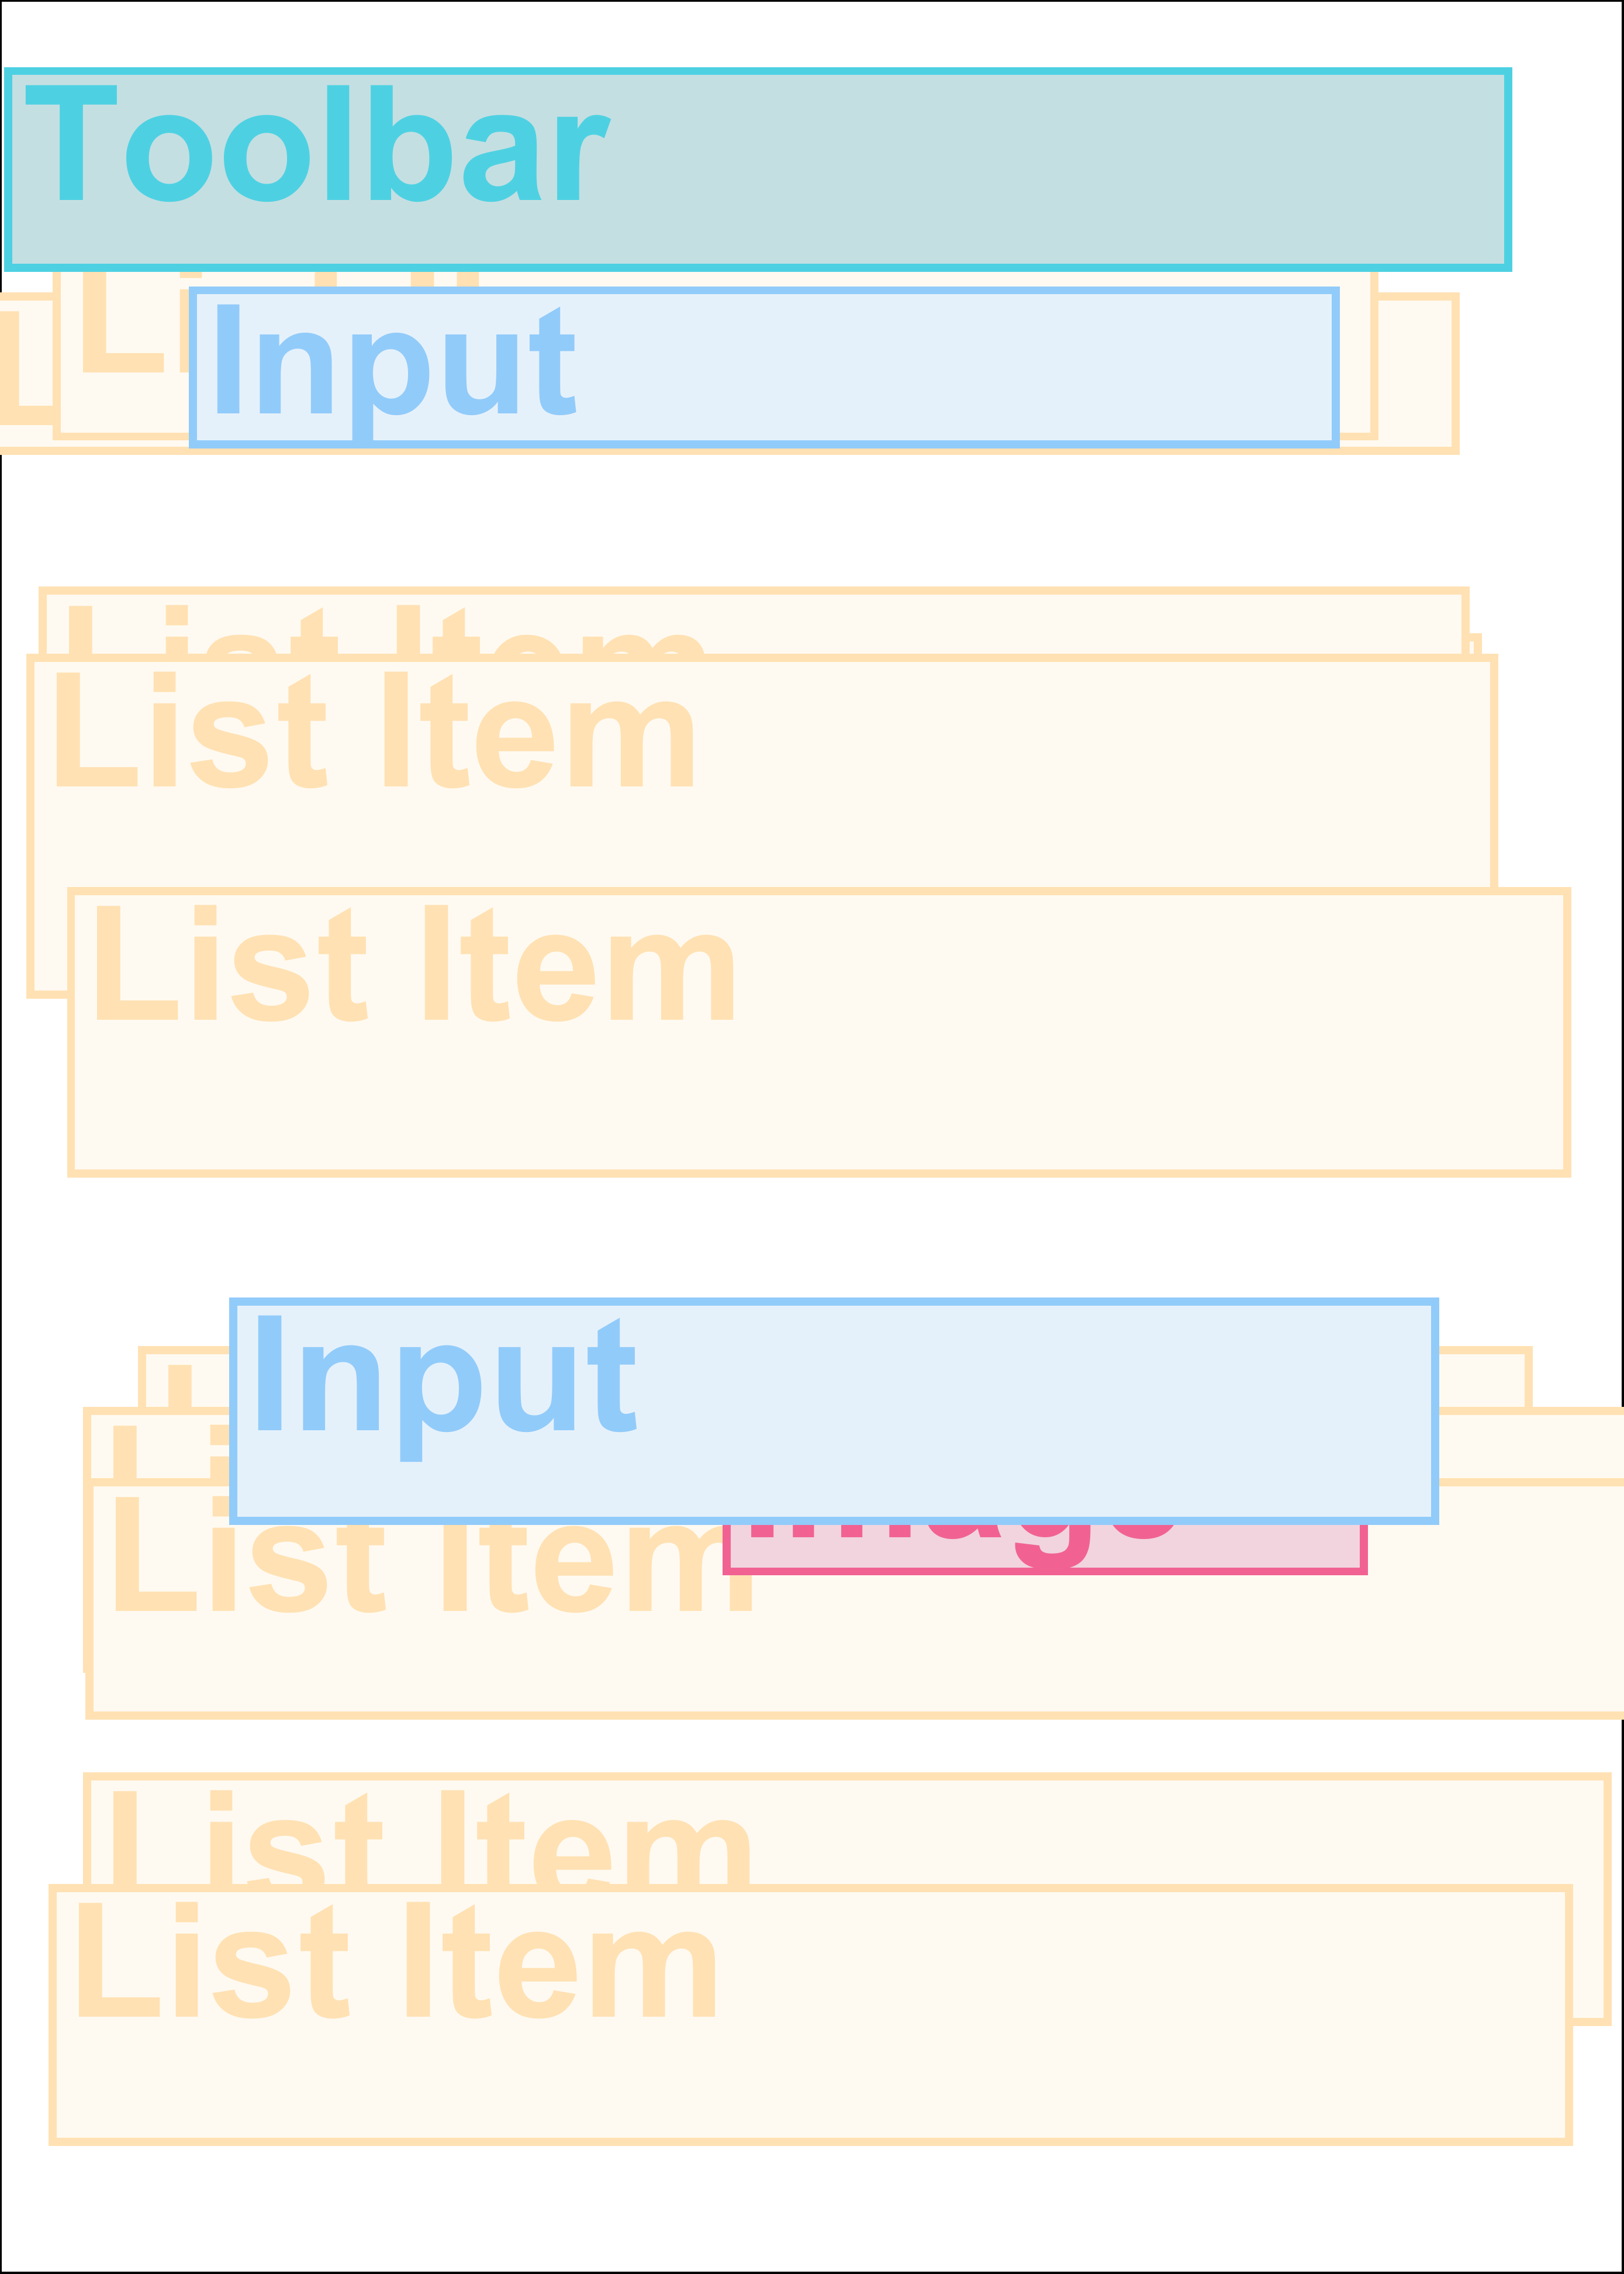}\\

\rotatebox{90}{\hspace{0.8cm} [9]} &
\includegraphics[width=\qualitativeComparisonWidthCoco]{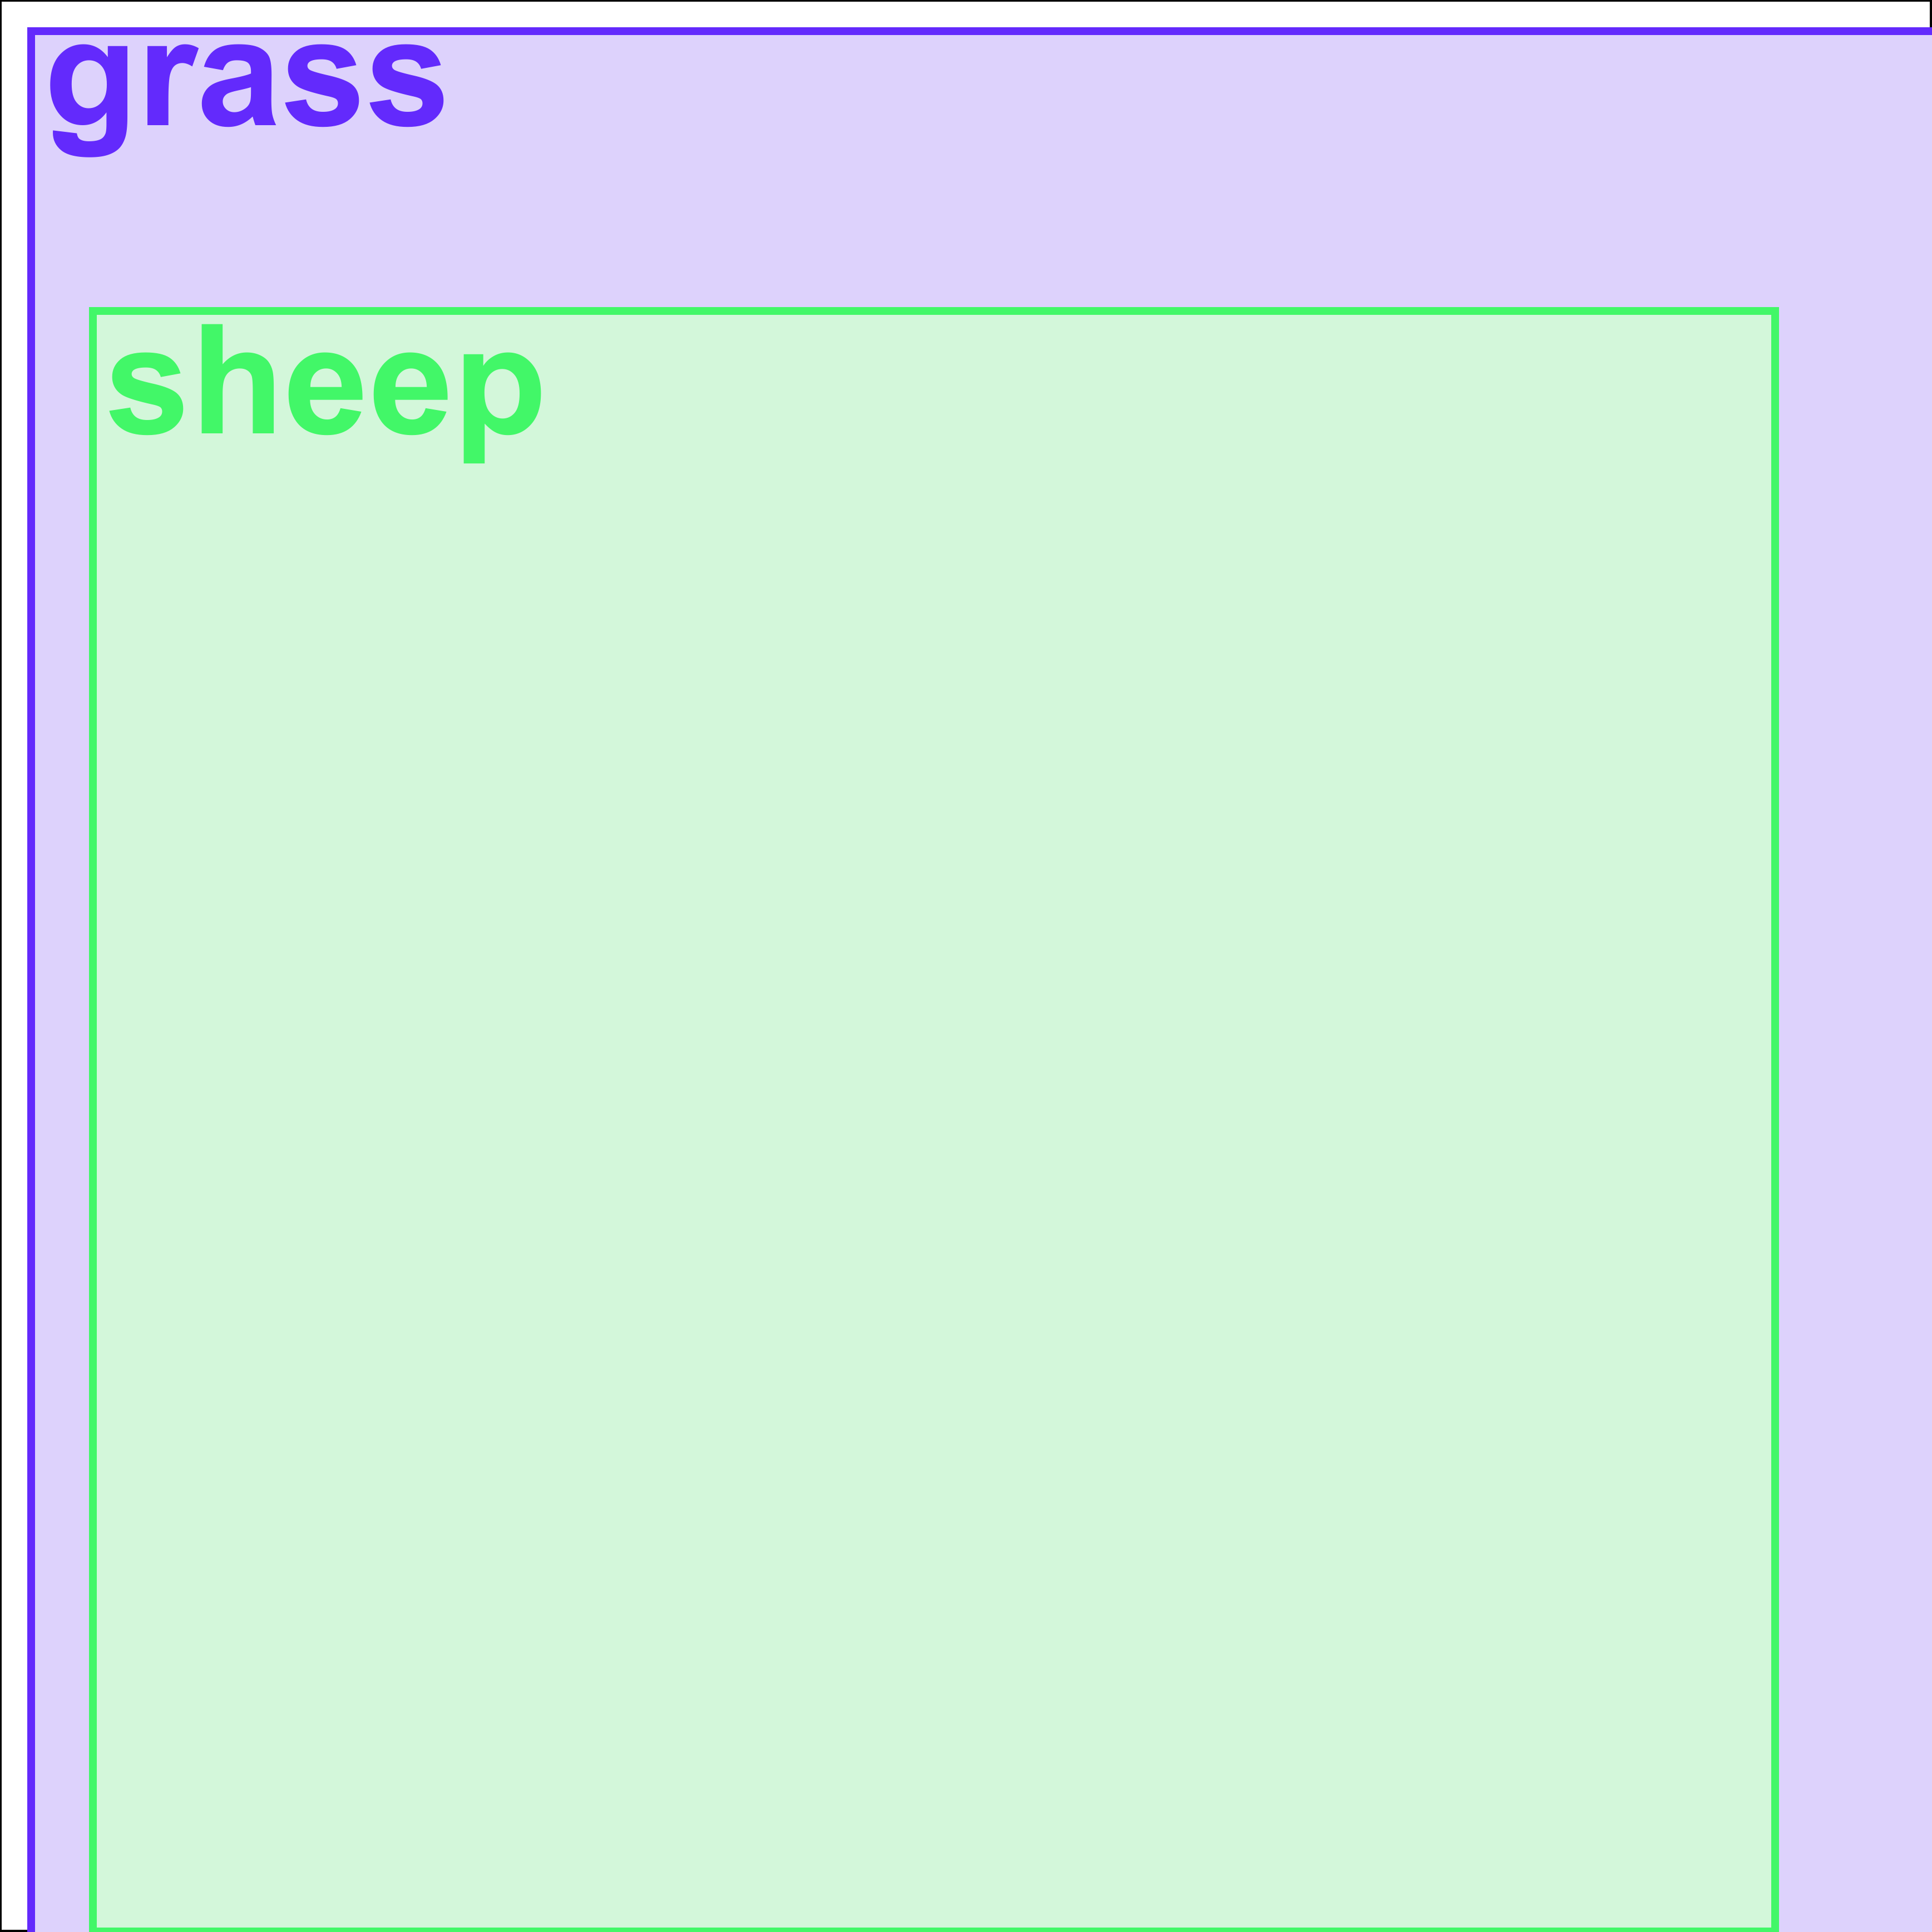} &
\includegraphics[width=\qualitativeComparisonWidthCoco]{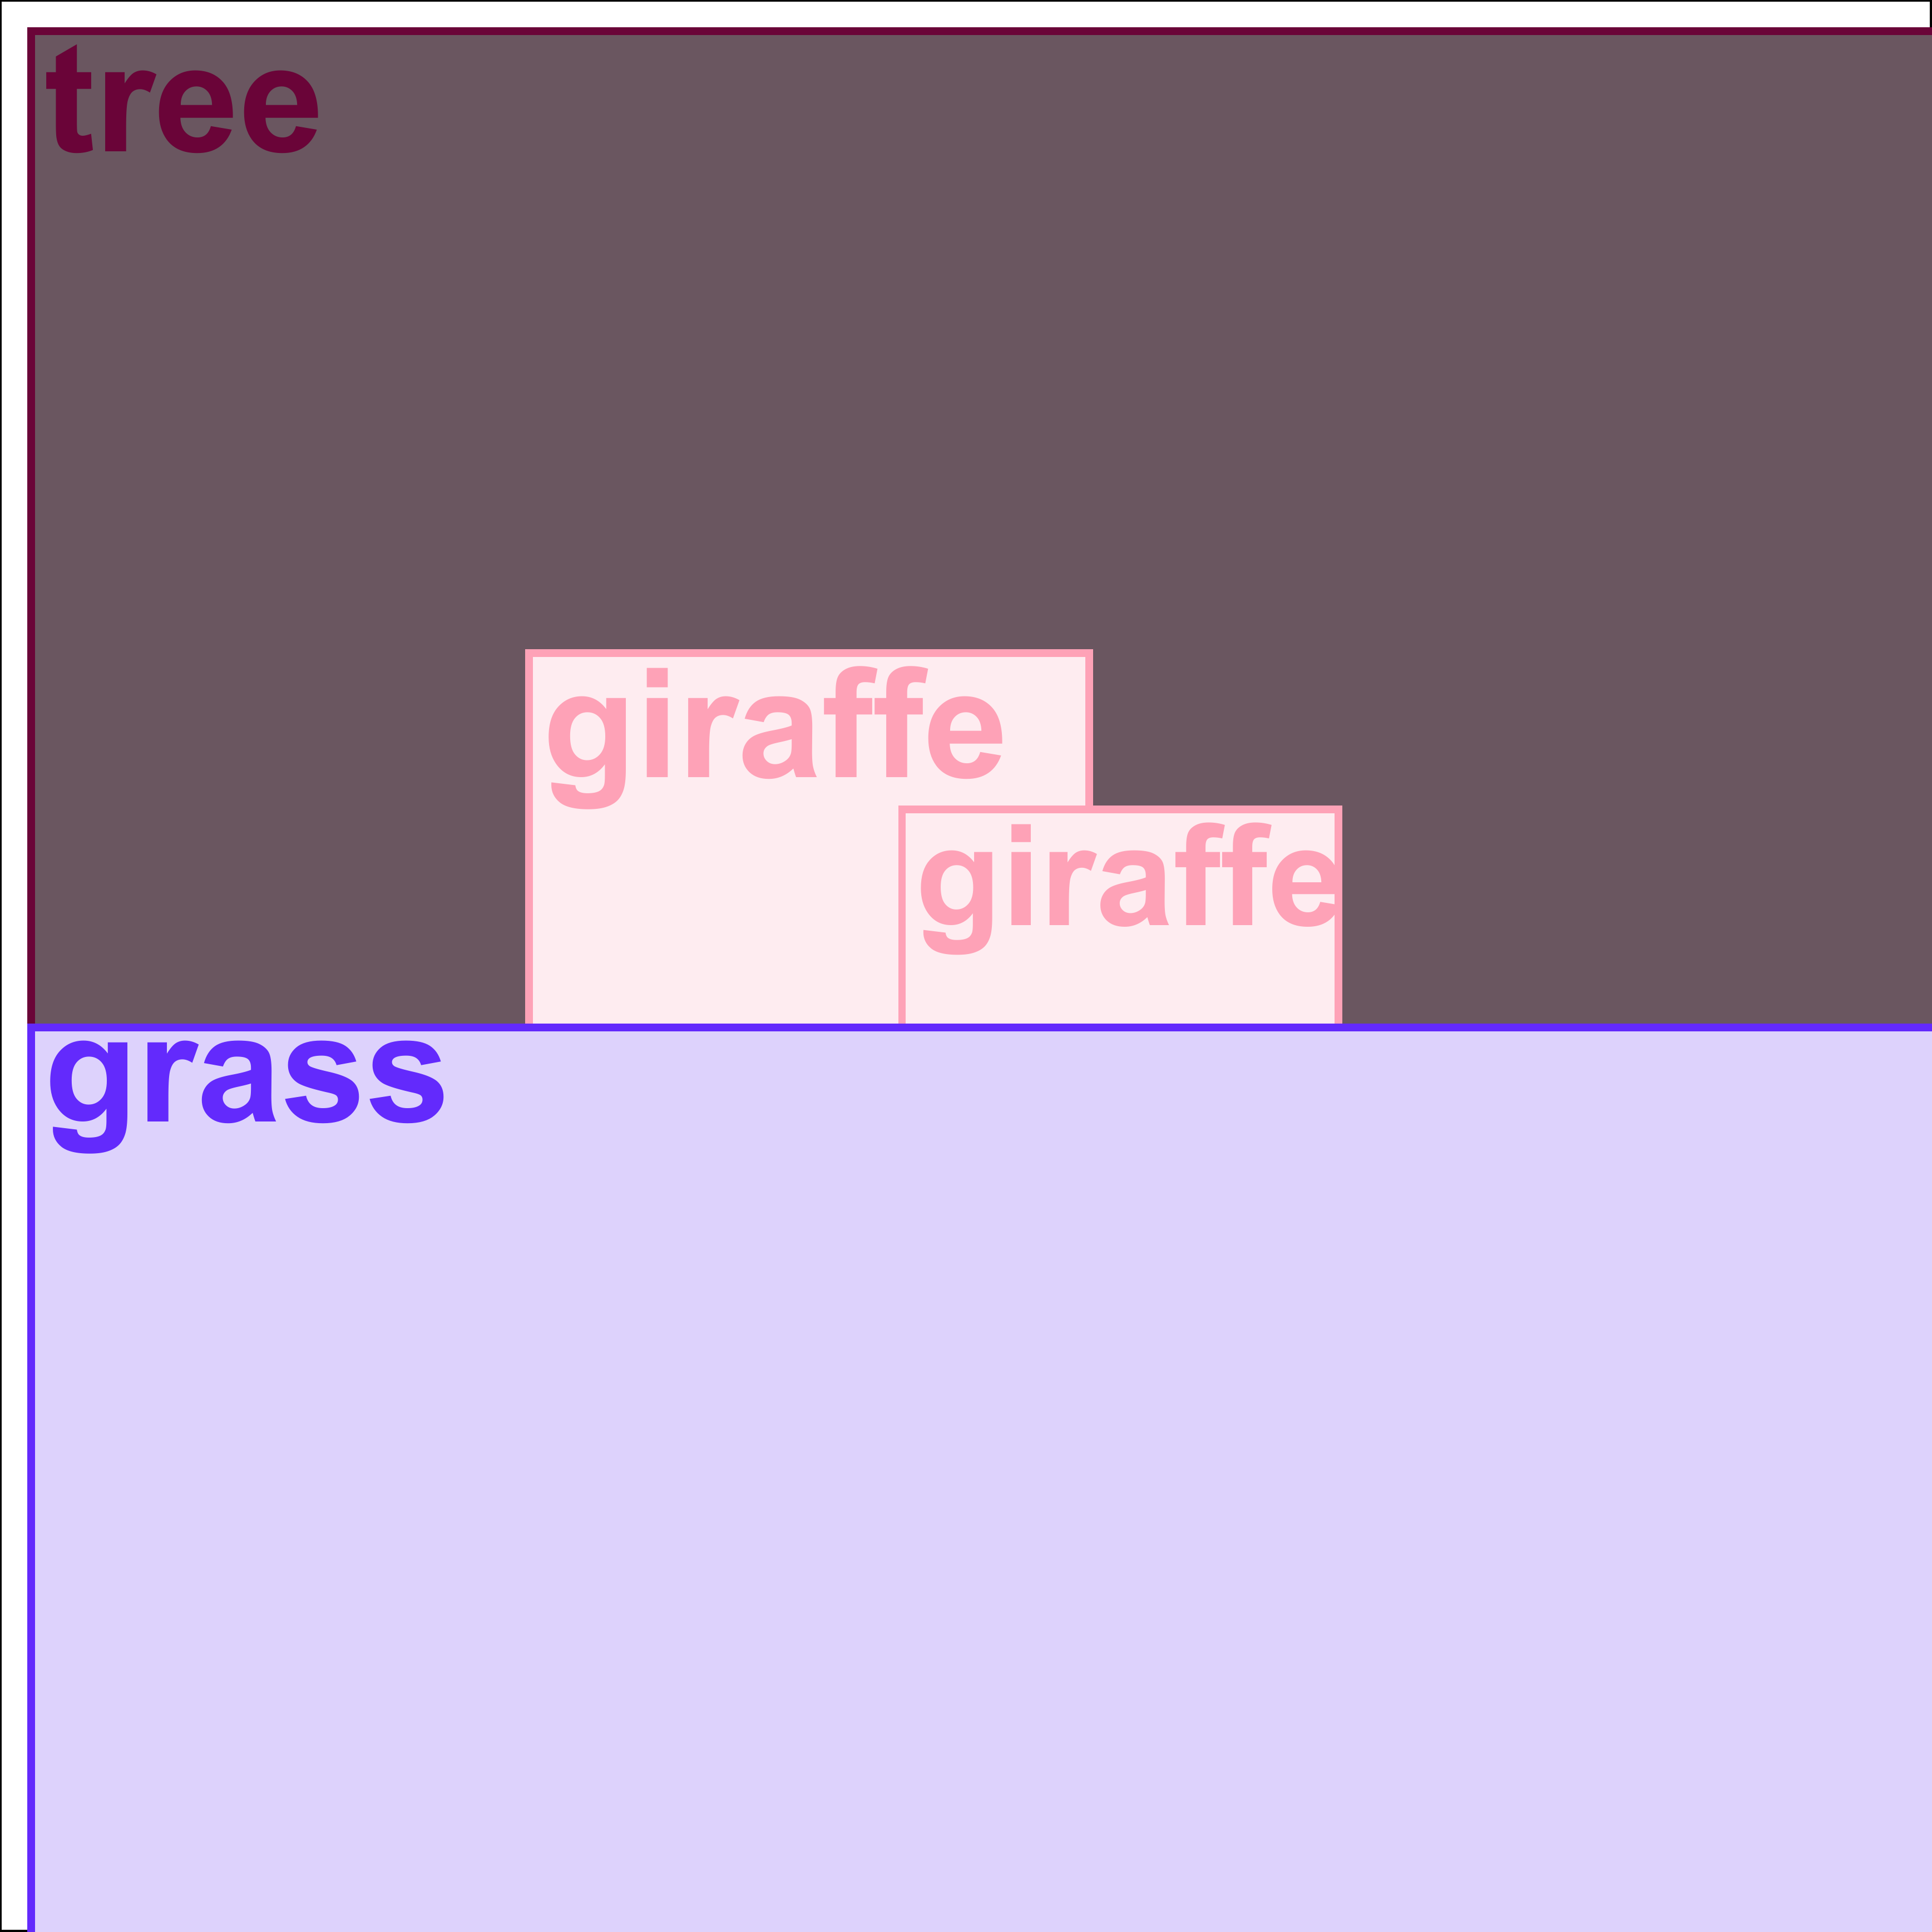} &
\includegraphics[width=\qualitativeComparisonWidth]{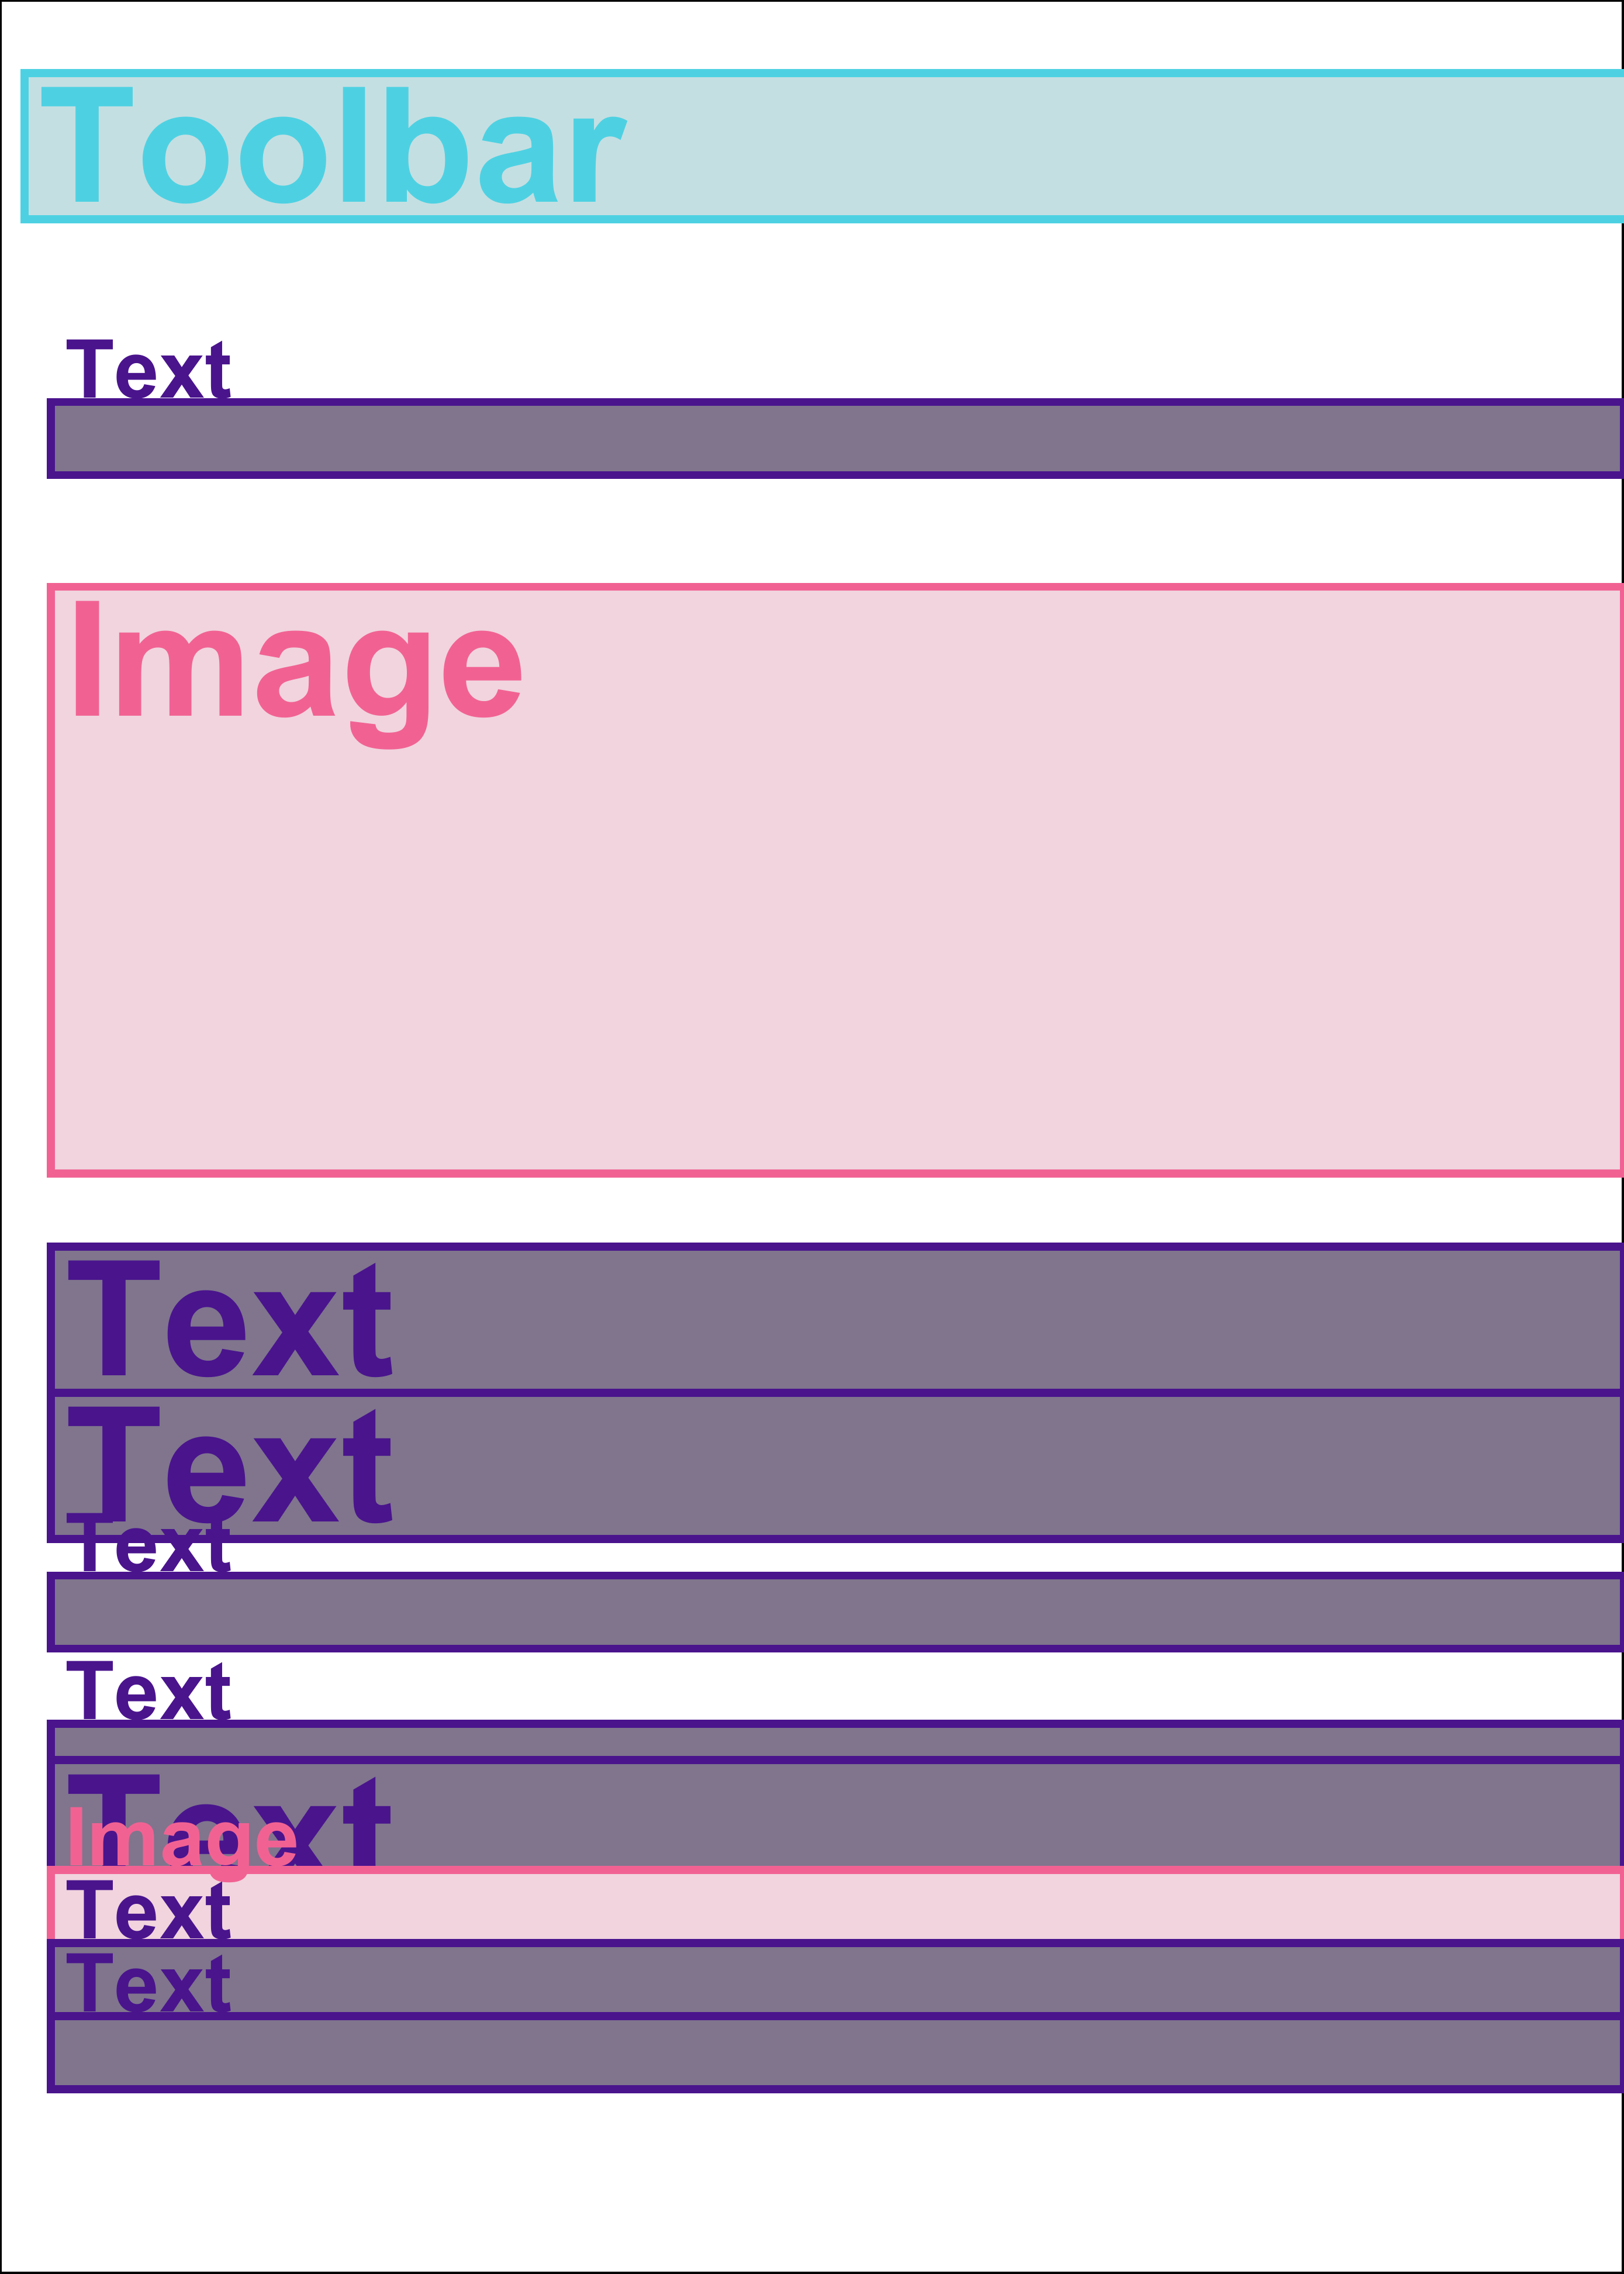} &
\includegraphics[width=\qualitativeComparisonWidth]{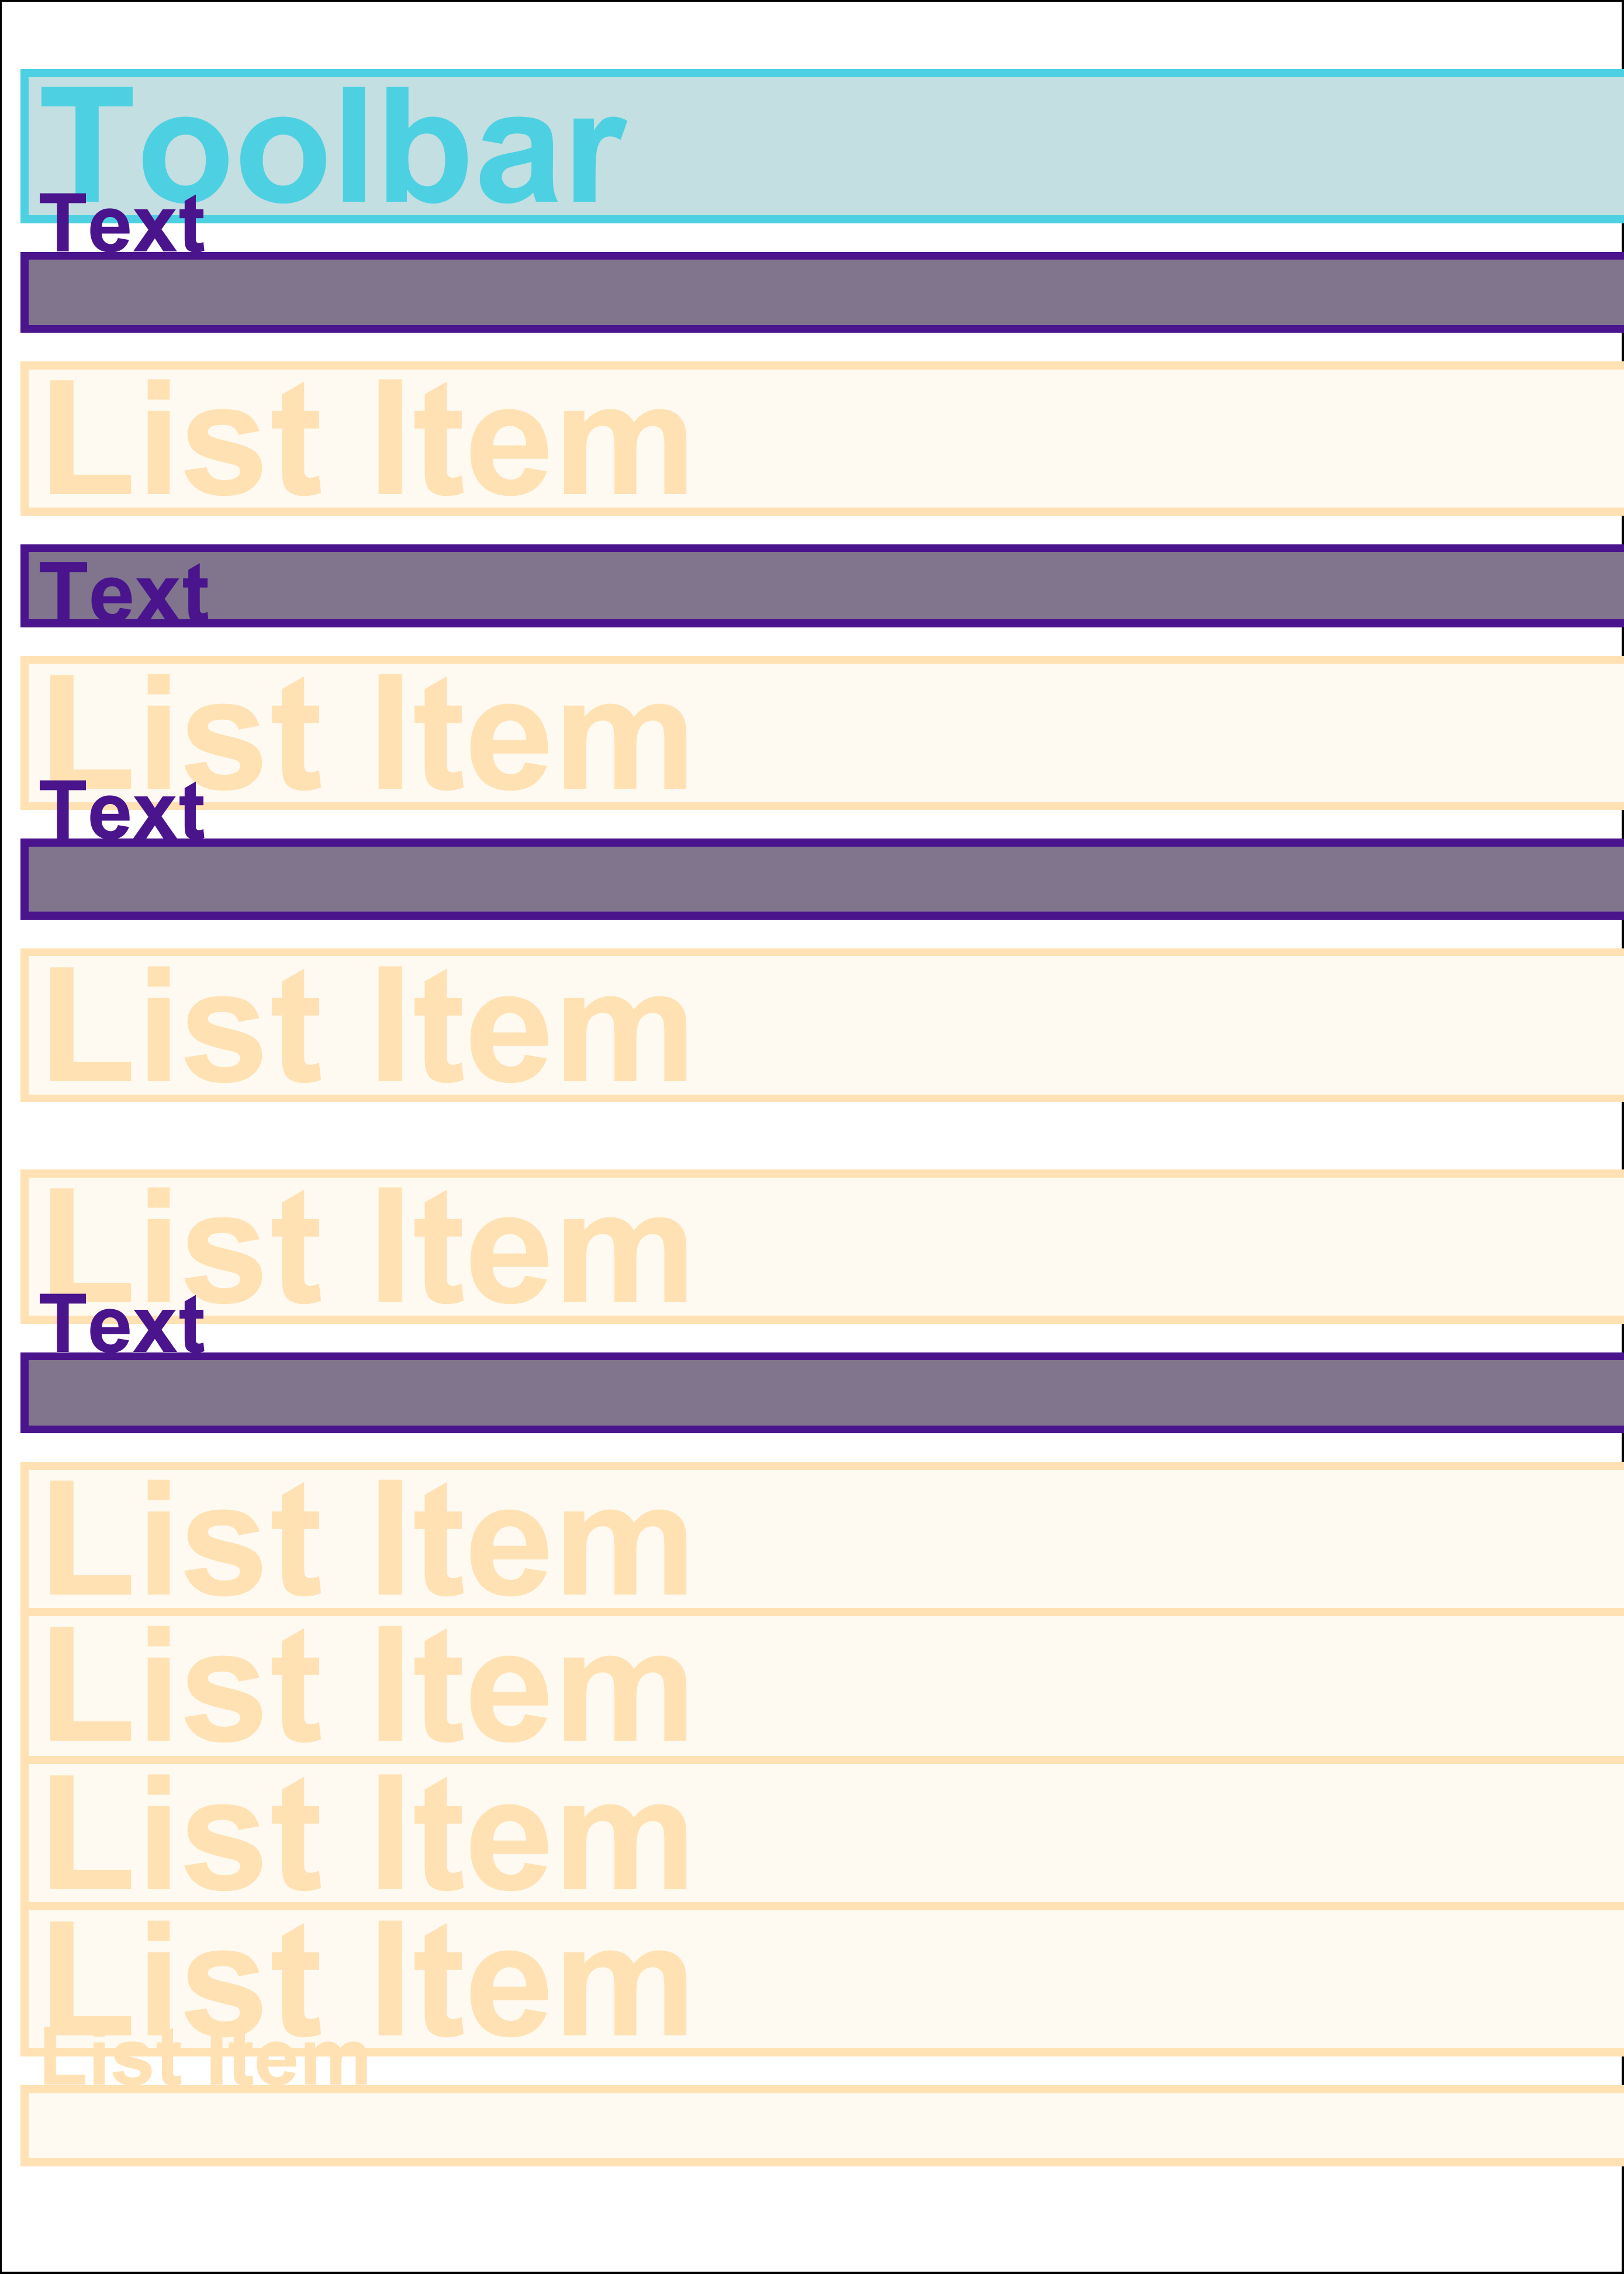} \\

\rotatebox{90}{\hspace{0.7cm} Ours} &
\includegraphics[width=\qualitativeComparisonWidthCoco]{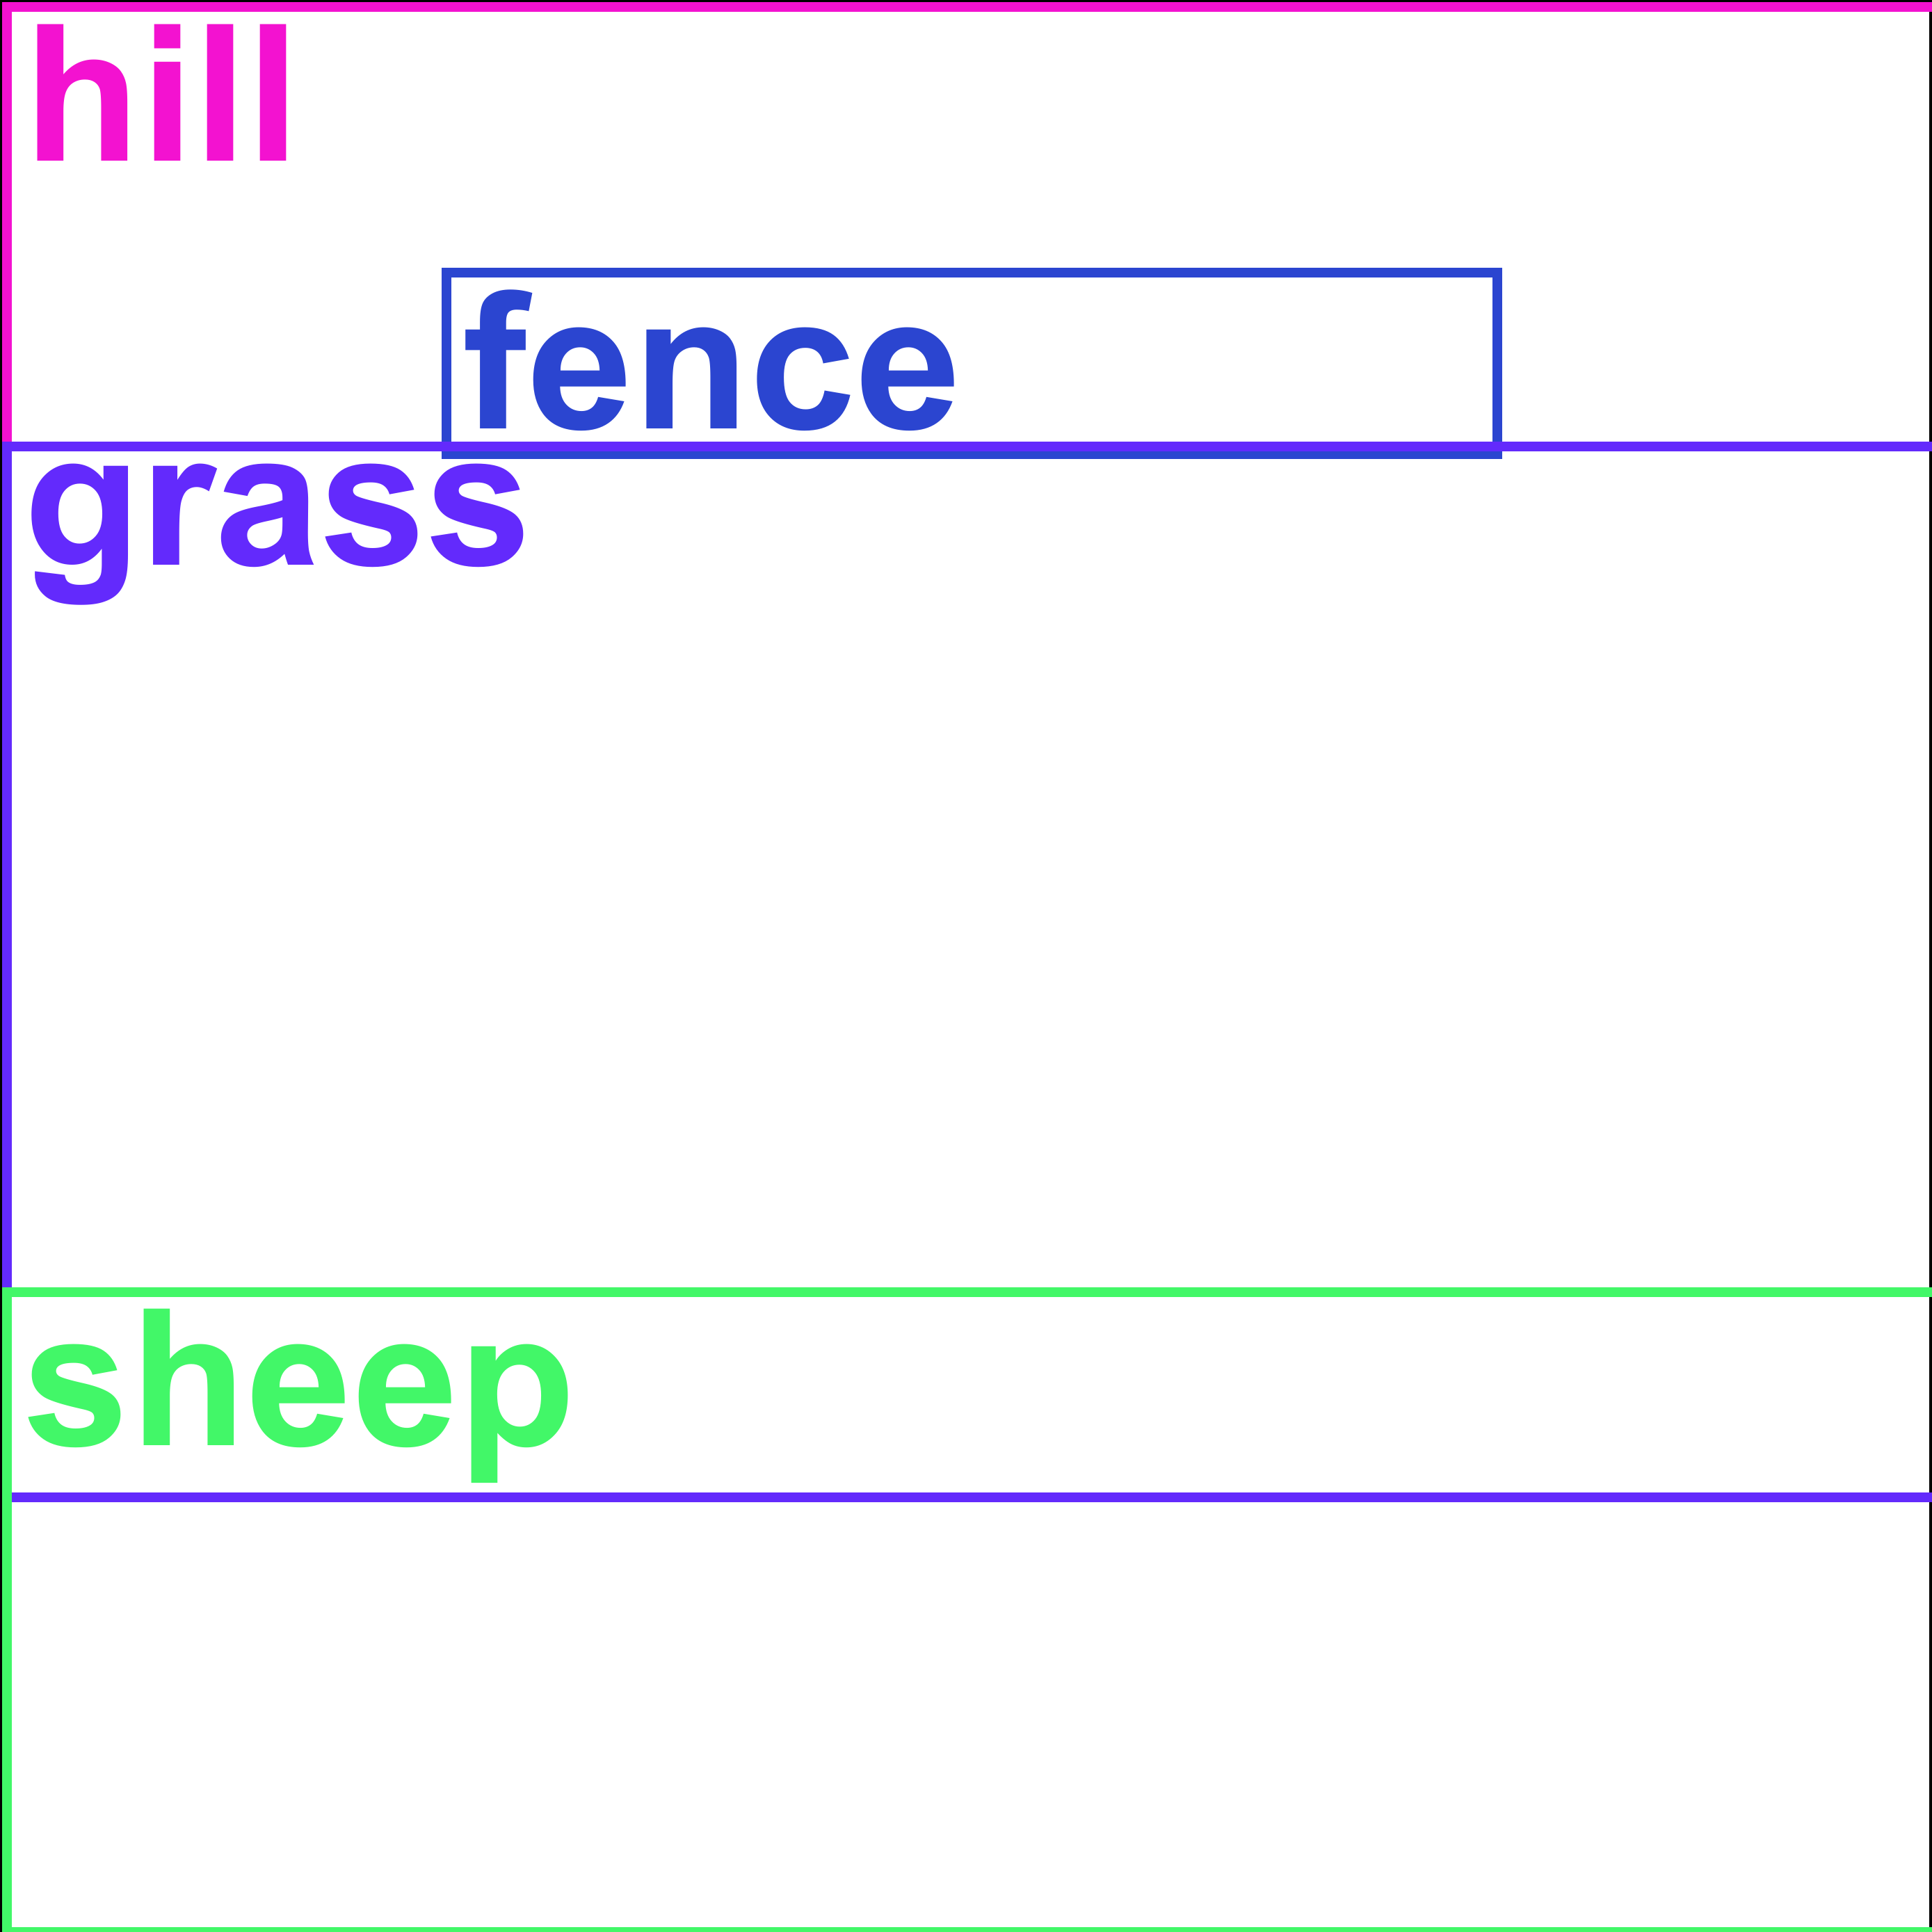} &
\includegraphics[width=\qualitativeComparisonWidthCoco]{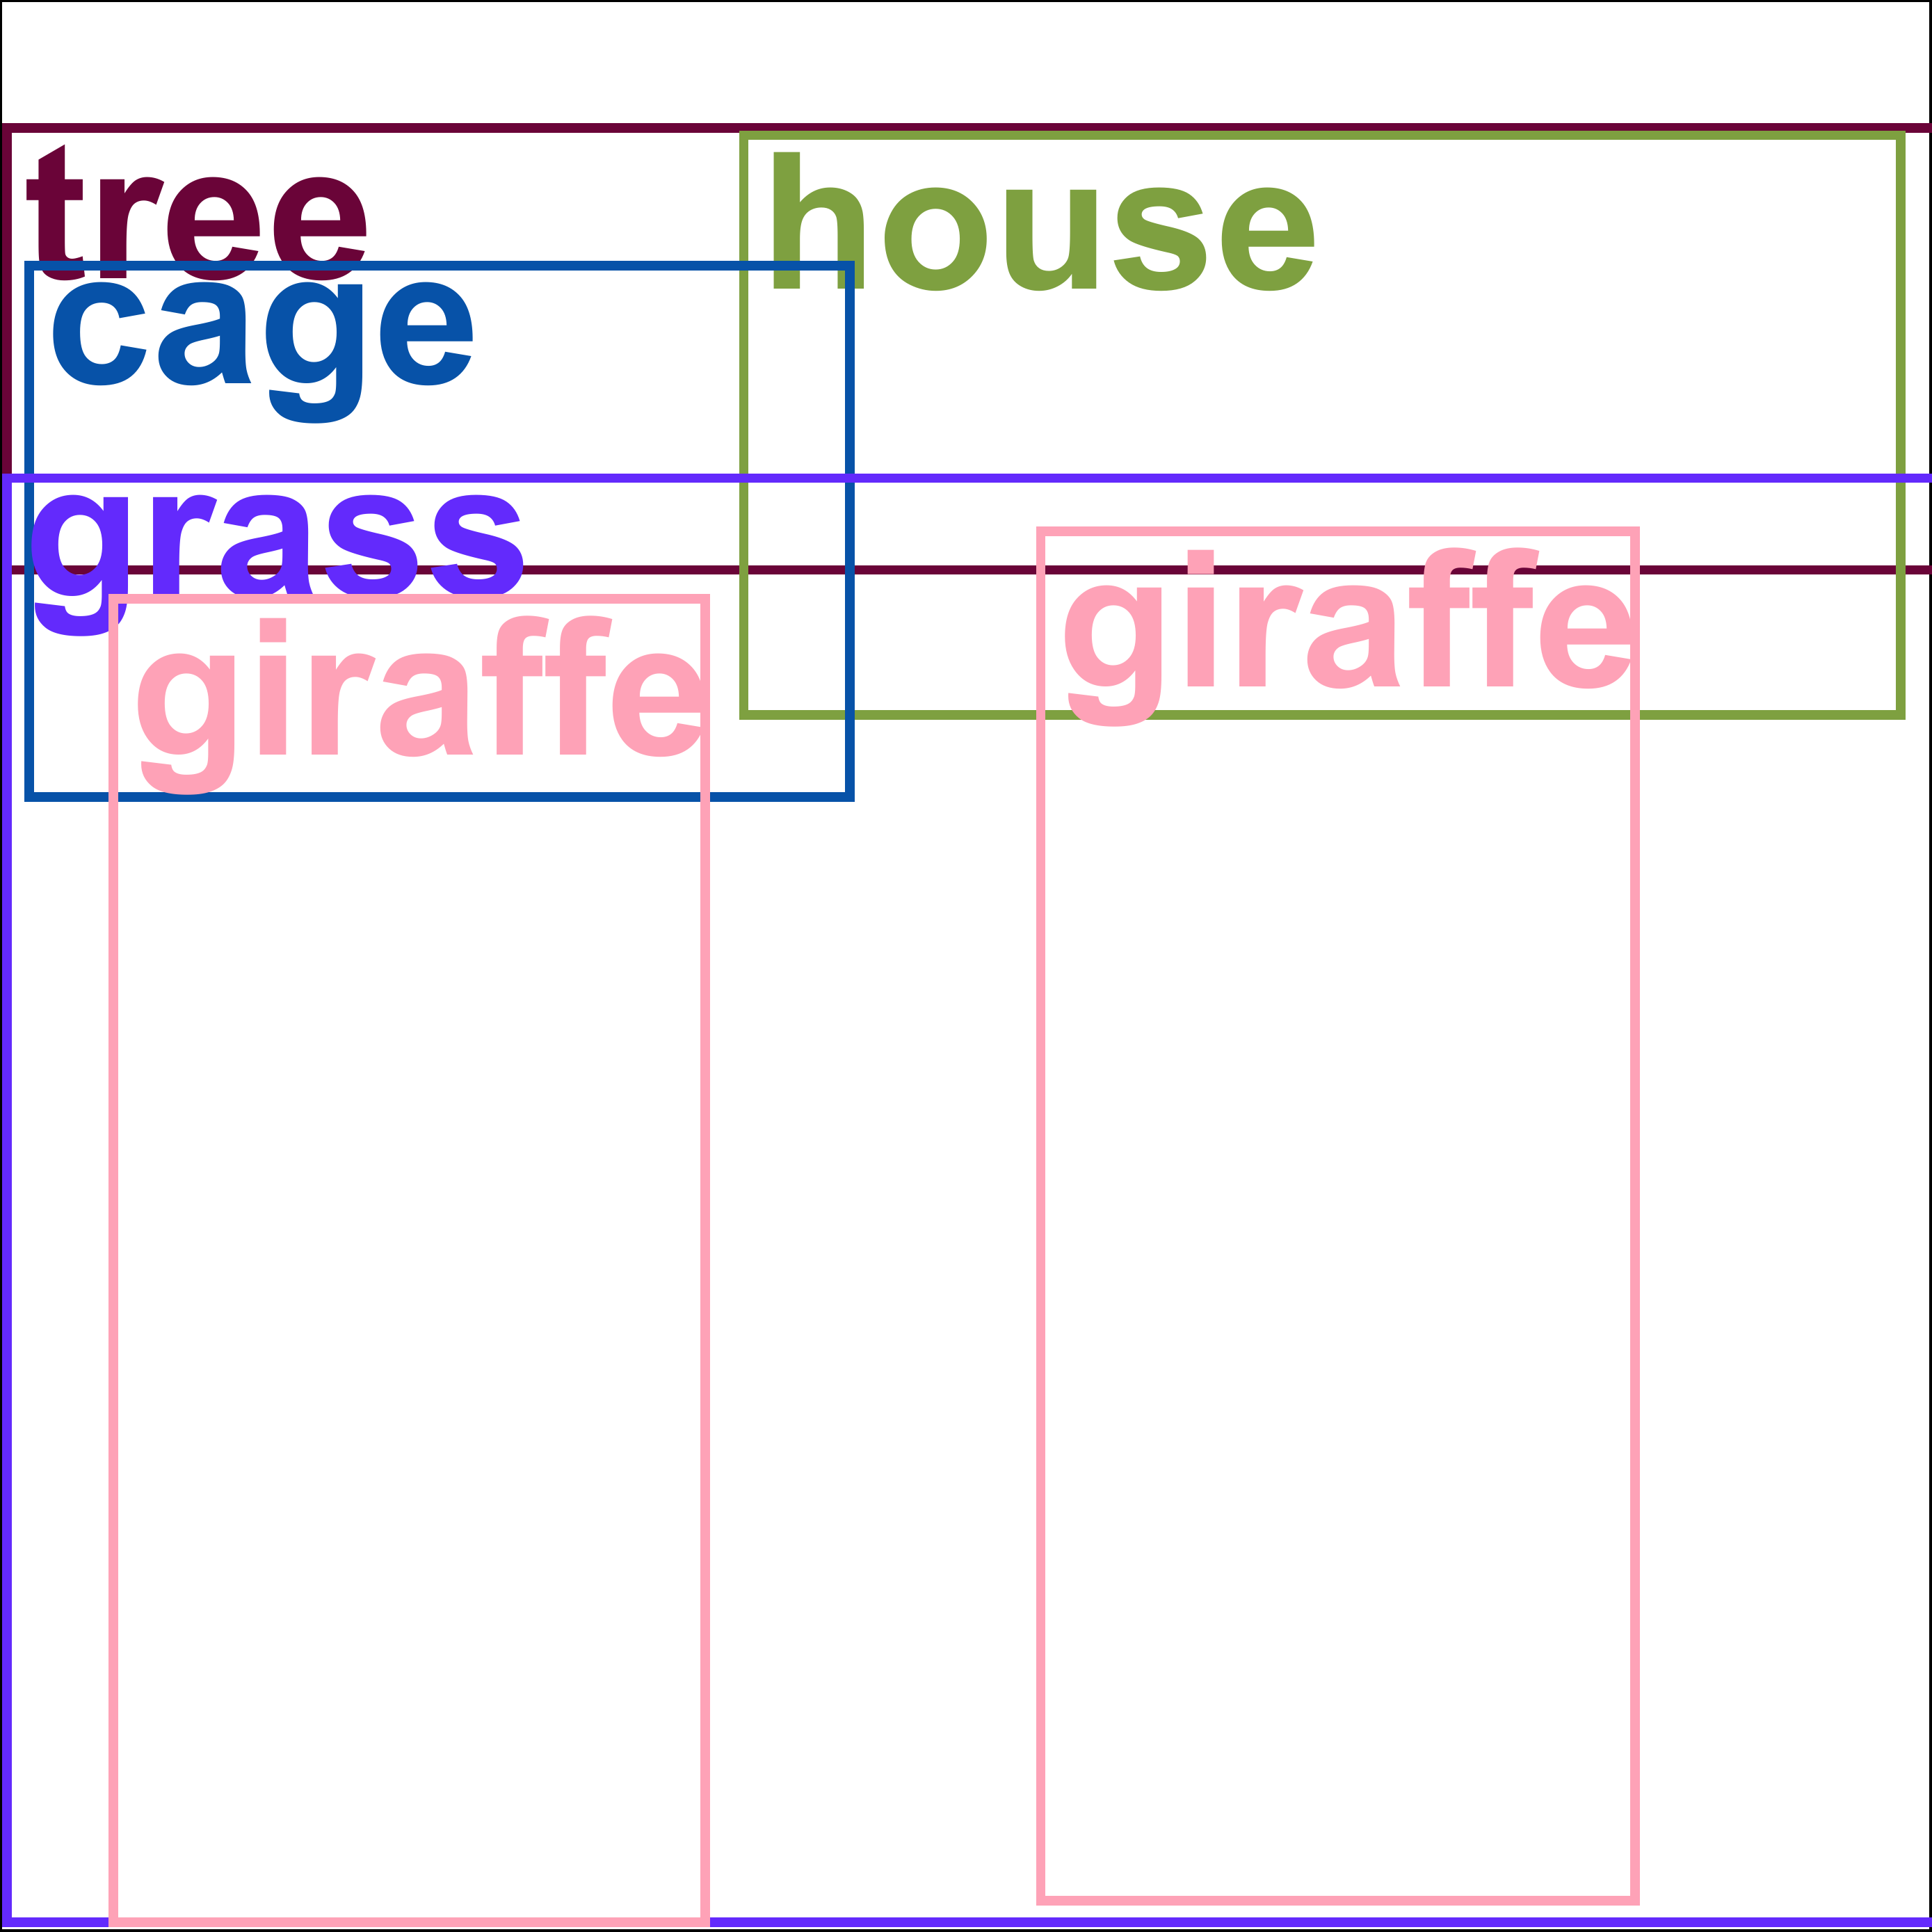} &
\includegraphics[width=\qualitativeComparisonWidth]{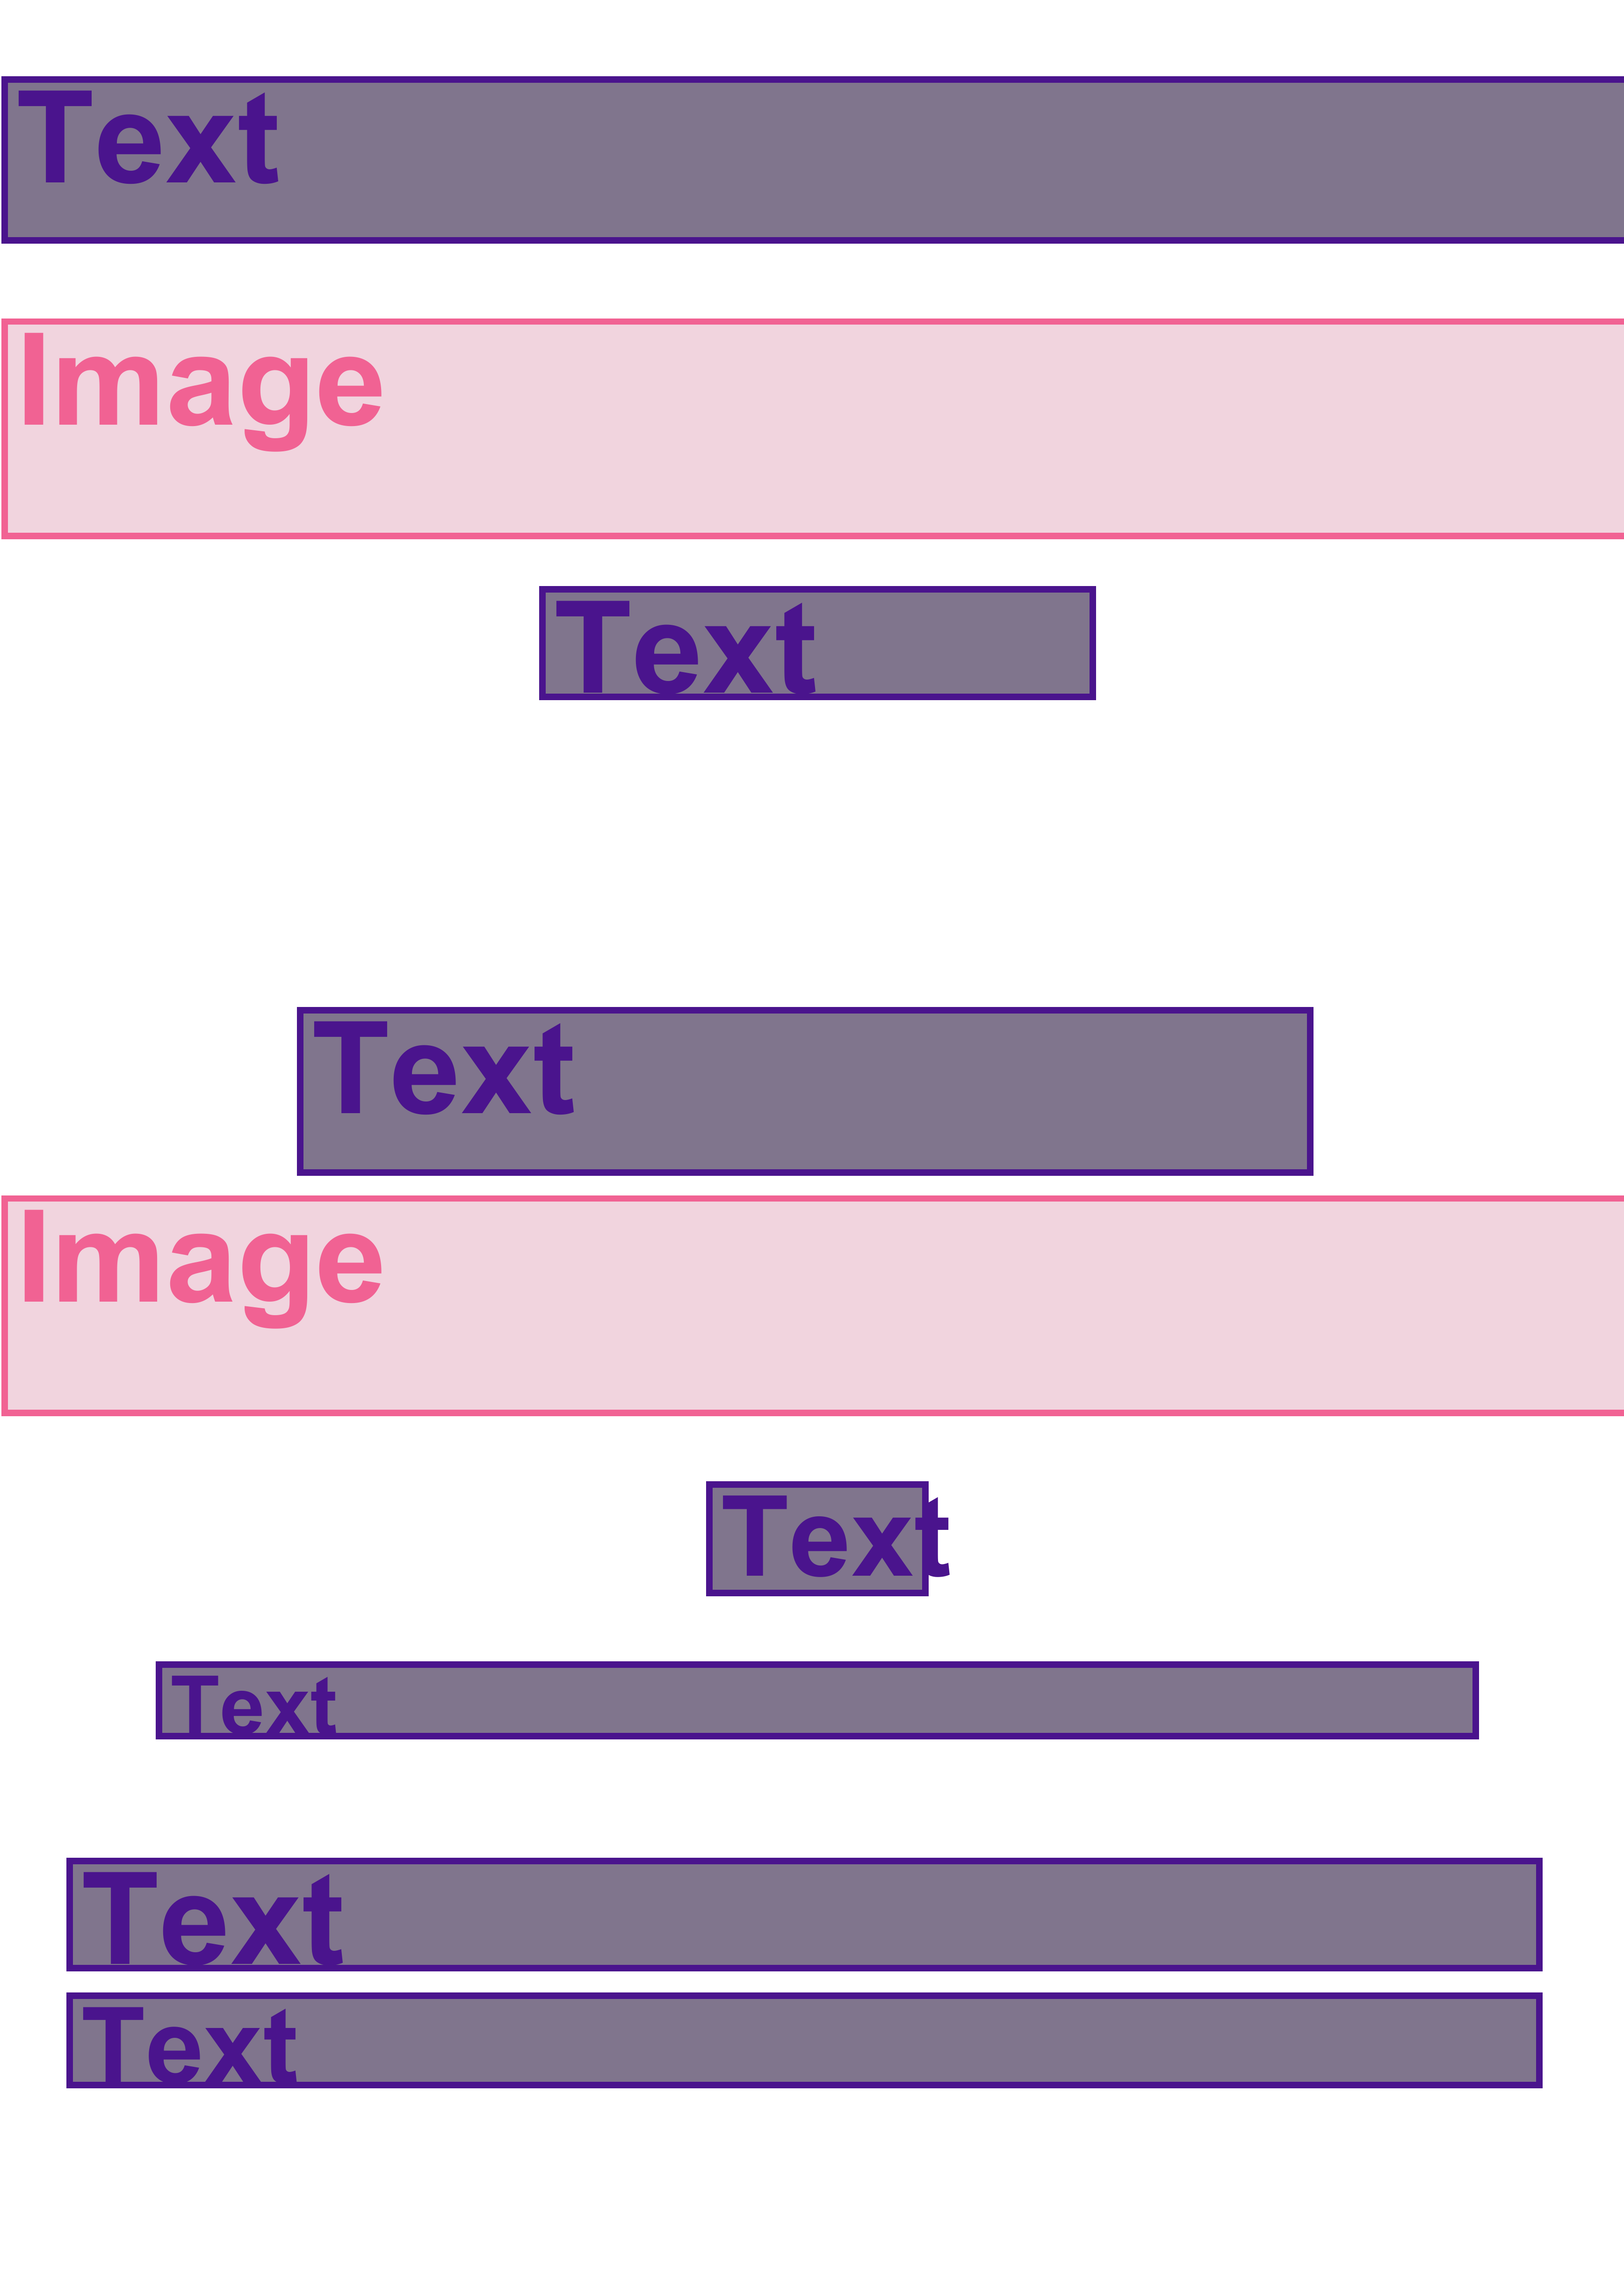} &
\includegraphics[width=\qualitativeComparisonWidth]{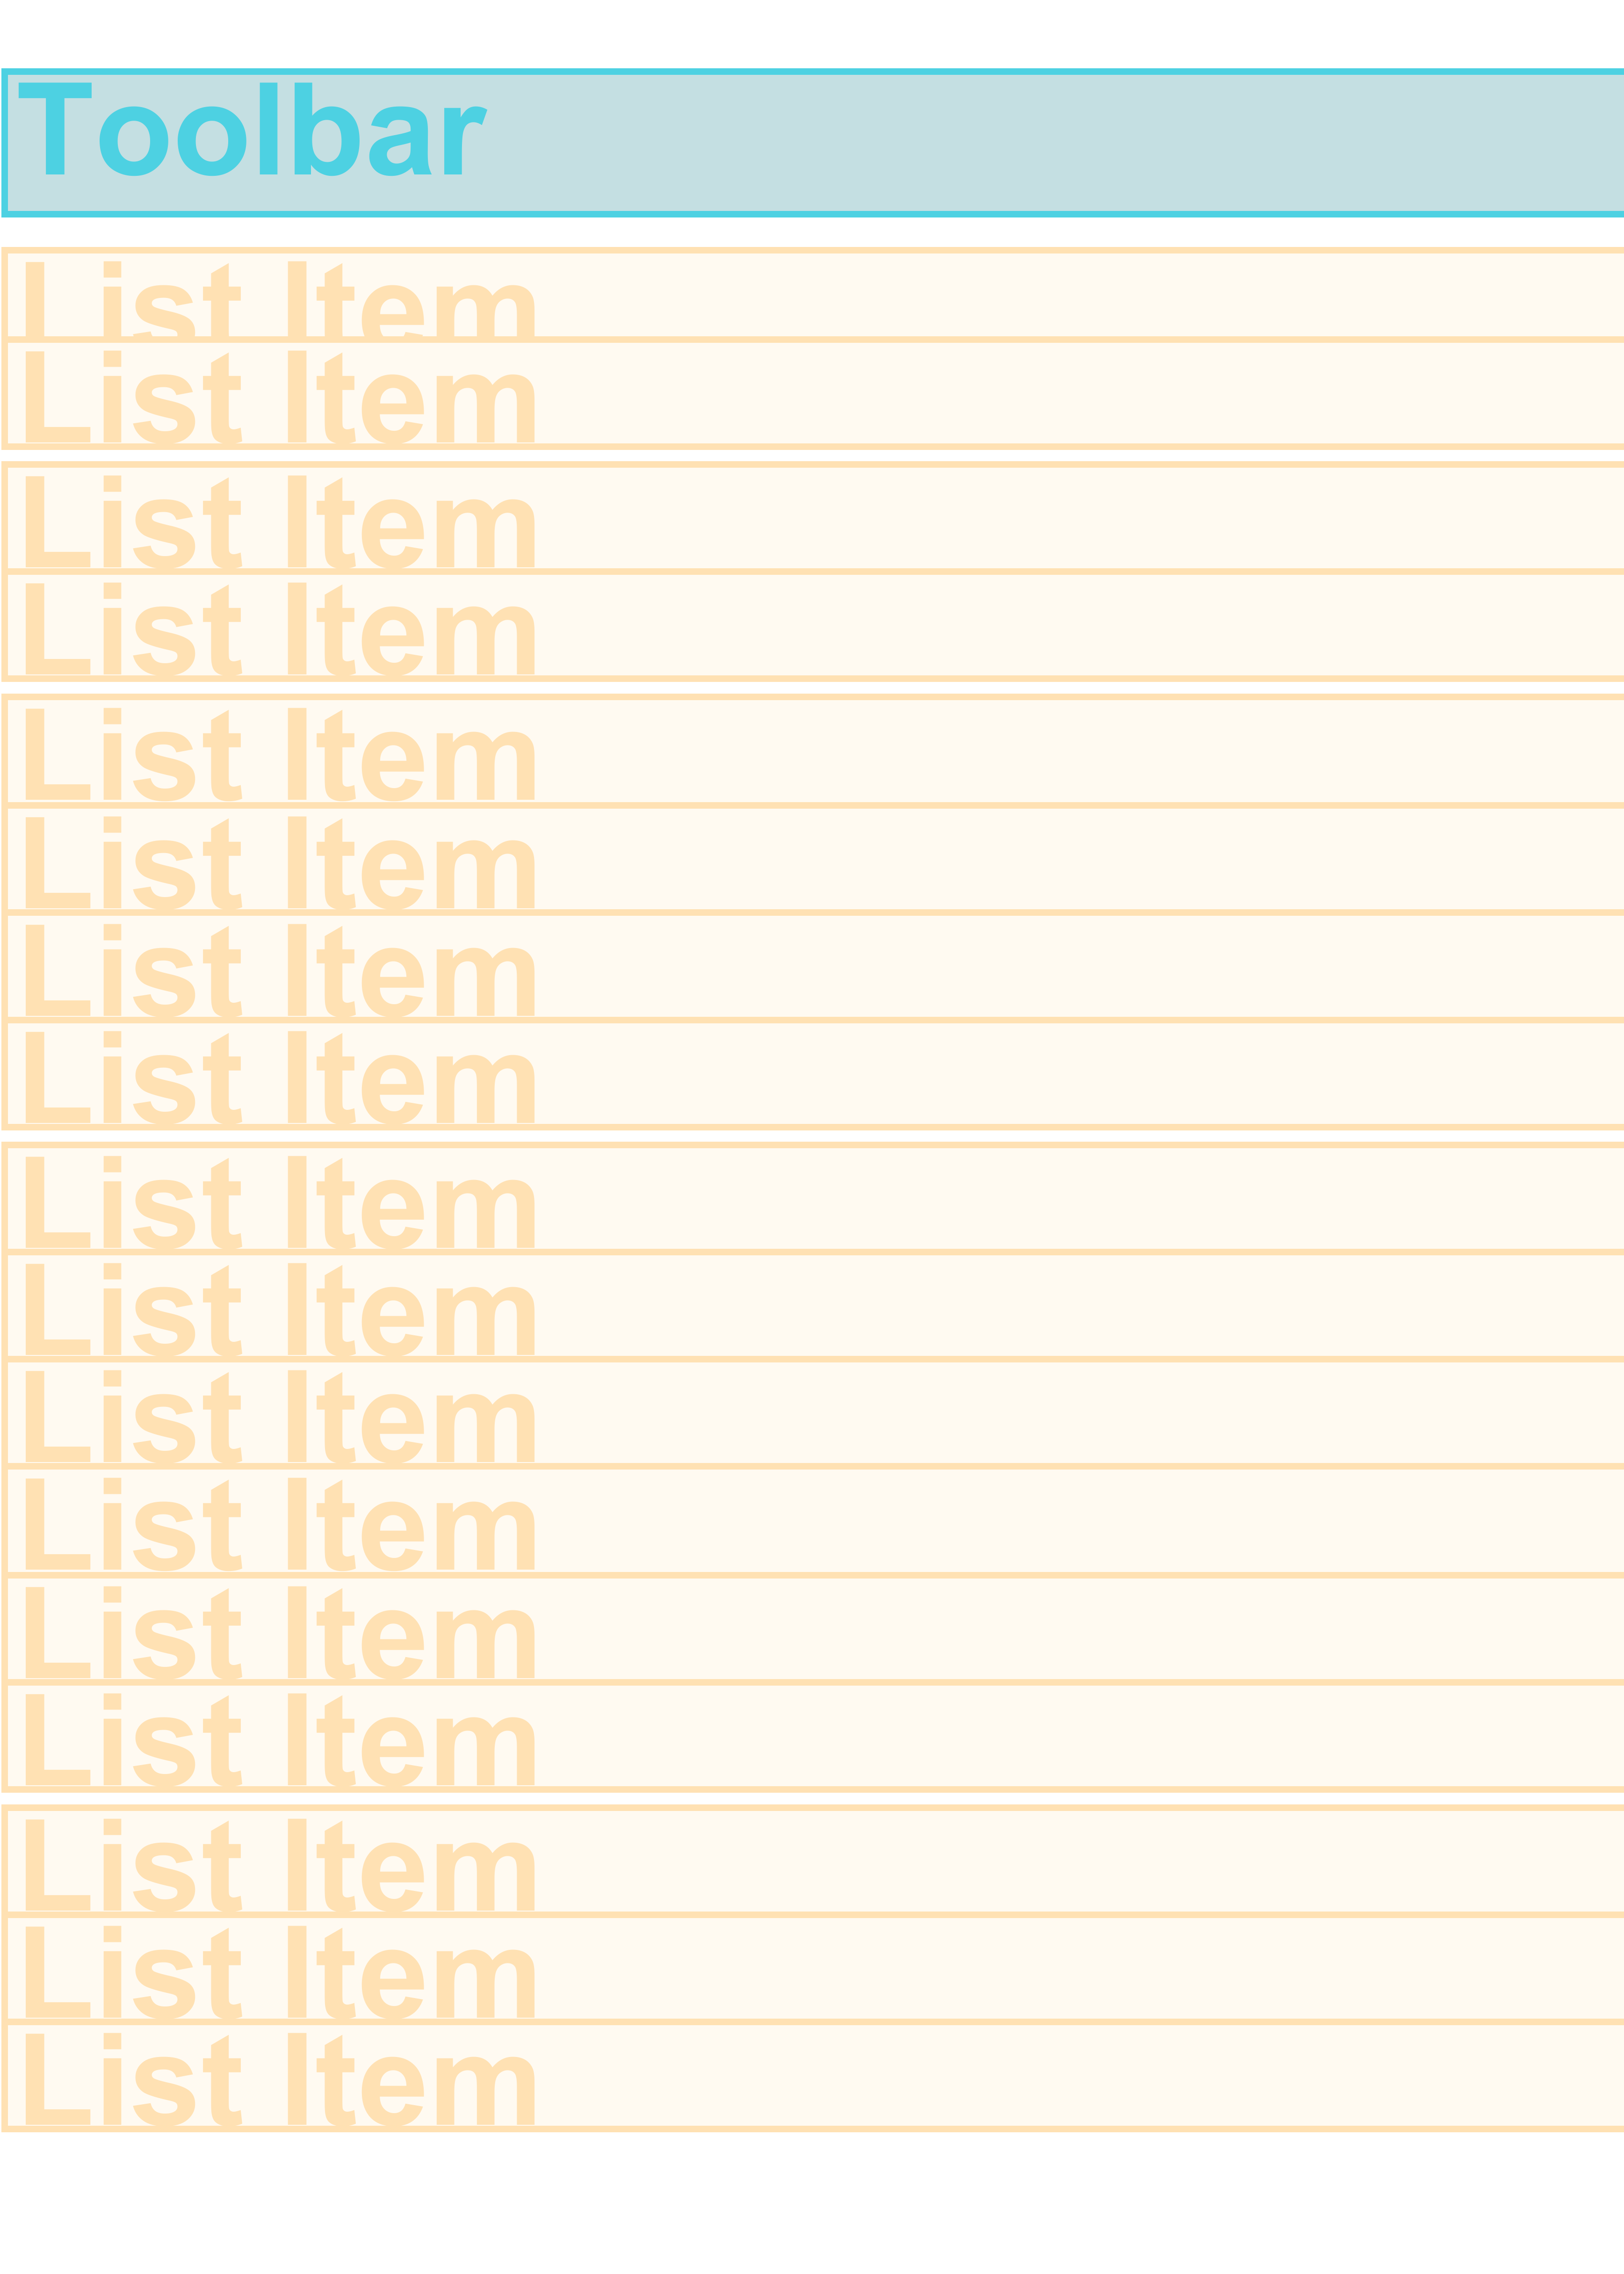} \\

\end{tabular}
    \caption{Comparison on COCO (left) and RICO (right).}
    \label{fig:figure_4_extension}
\end{figure}
